# Supplementary material for: The Ground State Electronic Energy of Benzene
Source: arXiv:2008.02678 ancillary file (2020-10-07)
Supplement: Supplementary file 1 [file si_benzene.pdf]

# Supporting Information:

# The Ground State Electronic Energy of Benzene

Janus J. Eriksen,[*,†] Tyler A. Anderson,[‡] J. Emiliano Deustua,[¶] Khaldoon Ghanem,[§] Diptarka Hait,[‖,⊥] Mark R. Hoffmann,[#] Seunghoon Lee,[@] Daniel S. Levine,[‖] Ilias Magoulas,[¶] Jun Shen,[¶] Norm M. Tubman,[‖] K. Birgitta Whaley,[‖] Enhua Xu,[△] Yuan Yao,[‡] Ning Zhang,[▽] Ali Alavi,[*,§,††] Garnet Kin-Lic Chan,[*,@] Martin Head-Gordon,[*,‖,⊥] Wenjian Liu,[*,‡‡] Piotr Piecuch,[*,¶,¶¶] Sandeep Sharma,[*,§§] Seiichiro L. Ten-no,[*,△] C. J. Umrigar,[*,‡] and Jürgen Gauss[*,‖‖]

†*School of Chemistry, University of Bristol, Cantock's Close, Bristol BS8 1TS, United Kingdom*

‡*Laboratory of Atomic and Solid State Physics, Cornell University, Ithaca, New York 14853, USA*

¶*Department of Chemistry, Michigan State University, East Lansing, Michigan 48824, USA*

§*Max-Planck-Institut für Festkörperforschung, 70569 Stuttgart, Germany*

‖*Kenneth S. Pitzer Center for Theoretical Chemistry, Department of Chemistry, University of California, Berkeley, California 94720, USA*

⊥*Chemical Sciences Division, Lawrence Berkeley National Laboratory, Berkeley, California 94720, USA*

#*Chemistry Department, University of North Dakota, Grand Forks, North Dakota 58202-9024, USA*

@*Division of Chemistry and Chemical Engineering, California Institute of Technology, Pasadena, California 91125, USA*

△*Graduate School of Science, Technology, and Innovation, Kobe University, 1-1 Rokkodai-cho, Nada-ku, Kobe 657-8501, Japan*

▽*Beijing National Laboratory for Molecular Sciences, Institute of Theoretical and Computational Chemistry, College of Chemistry and Molecular Engineering, Peking University, Beijing 100871, China*

††*Department of Chemistry, University of Cambridge, Cambridge CB2 1EW, United Kingdom*

‡‡*Qingdao Institute for Theoretical and Computational Sciences, Shandong University, Qingdao, Shandong 266237, China*

¶¶*Department of Physics and Astronomy, Michigan State University, East Lansing, Michigan 48824, USA*

§§*Department of Chemistry, The University of Colorado at Boulder, Boulder, Colorado 80302, USA*

‖‖*Department Chemie, Johannes Gutenberg-Universität Mainz, Duesbergweg 10-14, 55128 Mainz, Germany*

E-mail: janus.eriksen@bristol.ac.uk; a.alavi@fkf.mpg.de; gkc1000@gmail.com; mhg@cchem.berkeley.edu; liuwj@sdu.edu.cn; piecuch@chemistry.msu.edu; sandeep.sharma@colorado.edu; tenno@garnet.kobe-u.ac.jp; cyrusumrigar@gmail.com; gauss@uni-mainz.de

# 1 Geometry

The geometry of benzene used in our study is the MP2/6-31G* optimized structure from Ref. S1, cf. Table S1. For reference, the nuclear repulsion and Hartree-Fock energies are $E_{\mathrm{nuc}} = 203.15350971\ E_{\mathrm{H}}$ and $E_{\mathrm{HF}} = -230.721819131\ E_{\mathrm{H}}$, respectively.

**Table S1:** $C_6H_6$ (in Å).

| Atom | $x$ | $y$ | $z$ |
|---|---|---|---|
| C | 0.000000 | 1.396792 | 0.000000 |
| C | 0.000000 | −1.396792 | 0.000000 |
| C | 1.209657 | 0.698396 | 0.000000 |
| C | −1.209657 | −0.698396 | 0.000000 |
| C | −1.209657 | 0.698396 | 0.000000 |
| C | 1.209657 | −0.698396 | 0.000000 |
| H | 0.000000 | 2.484212 | 0.000000 |
| H | 2.151390 | 1.242106 | 0.000000 |
| H | −2.151390 | −1.242106 | 0.000000 |
| H | −2.151390 | 1.242106 | 0.000000 |
| H | 2.151390 | −1.242106 | 0.000000 |
| H | 0.000000 | −2.484212 | 0.000000 |

# 2 Main Results

Table S2 summarizes the results of the blind-challenge calculations shown in Fig. 1 of the main text. Methods are ordered by the final correlation energy.

**Table S2:** Summary of Fig. 1 from the main text.

| Method | $\Delta E/\mathrm{m}E_{\mathrm{H}}$ |
|---|---|
| ASCI | −860.0 |
| iCI | −861.1 |
| CCSDTQ | −862.4 |
| DMRG | −862.8 |
| FCCR | −863.0 |
| MBE-FCI | −863.0 |
| CAD-FCIQMC | −863.4 |
| AS-FCIQMC | −863.7 |
| SHCI | −864.2 |

# 3 MBE-FCI

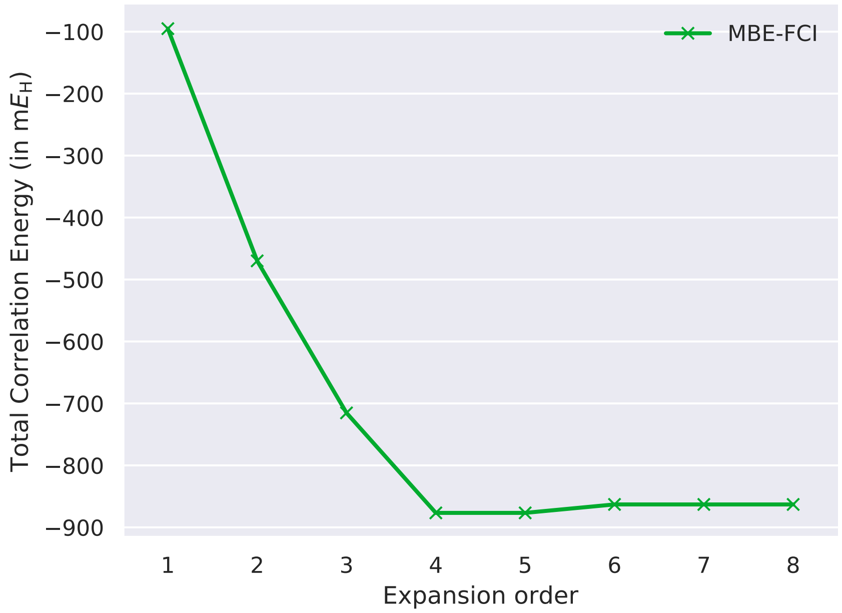


**Figure S1:** MBE-FCI results.

In MBE-FCI theory,[S2–S5] the complete set of MOs for a given system is divided into a reference space and an expansion space. An MBE-FCI expansion in the latter of these spaces hence recovers the residual correlation not captured by an FCI calculation constrained to the former. The MBE-FCI calculation of the present work is presented in Figure S1, as performed in an embarrassingly parallel manner using the open-source `PyMBE` code[S6] on Intel Xeon E5-2697v4 (Broadwell) hardware (36 cores @ 2.3 GHz, 3.56 GB/core). The calculation was performed in a basis of localized Pipek-Mezey MOs[S7] with a (6$e$,6o) reference space consisting of the $\pi$- and $\pi^*$-orbitals and electrons. The final correlation energy is $\Delta E_{\text{MBE-FCI}} = -863.03$ m$E_{\text{H}}$.

In the course of preparing the code for running high-accuracy MBE-FCI calculations on the benzene molecule, a new screening protocol was implemented. At each order, MOs are screened away from the full expansion space according to their relative (absolute) magnitude, which in turn leads to a reduced number of increment calculations at the orders to follow.

Specifically, only the MOs of the expansion space (at any given order) that give rise to the numerically largest increments will be retained at the following order. For the calculation of the present work, the percentages of the expansion space retained ($a_{\text{retain}}$) alongside the number of individual CASCI calculations at any given order ($K_{\text{CASCI}}$) are presented in Table S3. In addition, a number of optimizations were made to the code base. Most crucially, a new pruning scheme was introduced to make sure that only non-redundant increments are stored in memory throughout the total MBE-FCI calculation. For instance, once the $i$th MO gets screened away from the expansion space, all increments at lower orders, which reference this MO, are not needed anymore and may thus be pruned. This allows for significantly larger problem sizes to be treated by the method. As such, the limiting factor in converging MBE-FCI even tighter for the problem at hand, that is, screening less throughout the expansion, is related to available computer ressources rather than physical memory.

**Table S3:** MBE-FCI calculation details.

| Order | $a_{\text{retain}}$/% | $\Delta E$/m$E_{\text{H}}$ | $K_{\text{CASCI}}$ |
|---|---|---|---|
| 1 | 100.0 | −95.1132 | 102 |
| 2 | 100.0 | −469.884 | 5,151 |
| 3 | 100.0 | −715.265 | 171,700 |
| 4 | 100.0 | −876.637 | 4,249,575 |
| 5 | 100.0 | −876.624 | 83,291,670 |
| 6 | 50.0 | −862.988 | 1,346,548,665 |
| 7 | 25.0 | −863.027 | 115,775,100 |
| 8 | 12.5 | −863.027 | 495 |

# 4 DMRG

For details on DMRG theory, please see a number of contemporary reviews on the topic.[S8–S10] All DMRG calculations were performed using an unmodified version of the `BLOCK` code (v1.5),[S11–S15] executed through the `PySCF` program,[S16–S18] on Intel Xeon CPU E5-2680v4 (28-36 cores @ 2.4 GHz, 9.85 GB/core) and Xeon Gold 6130 (32 cores @ 2.1 GHz, 6.0 GB/-core) nodes. Calculations were run in parallel on 100-200 cores. Maximum total memory

usage was estimated at 1.15 Tb in total across all cores; this includes replicated data on the cores. We used the standard procedures described in Ref. S15, including (i) Edminston-Ruedenberg split-localization of orbitals,[S19] (ii) and the use of the genetic algorithm option in `BLOCK` to order the orbitals. The forward schedule was carried out up to a maximum bond dimension of $M = 7000$, then the backward schedule was carried out to obtain fully converged results for extrapolation back down to $M = 1000$. We obtained our initial integral file from the Umrigar group for the blind challenge and used these for the DMRG calculations. As we found out subsequently, the integral file corresponded to optimized SHCI orbitals. As this makes the results more complicated to reproduce, we provide the full integral file at `https://github.com/seunghoonlee89/SI-benzene-paper-DMRG`. We also verified on some smaller runs that using CCSD natural orbitals gave similar energies. The results from the backwards schedule of DMRG are listed in Table S4.

**Table S4:** DMRG correlation energy ($E$ in m$E_{\mathrm{H}}$) and discarded weights ($w$) with the backwards schedule.

| $M$ | 1000 | 2000 | 3000 | 4000 | 5000 | 6000 | $\infty$ |
|---|---|---|---|---|---|---|---|
| $w$ | $5.3 \times 10^{-5}$ | $2.9 \times 10^{-5}$ | $2.1 \times 10^{-5}$ | $1.6 \times 10^{-5}$ | $1.3 \times 10^{-5}$ | $1.0 \times 10^{-5}$ | |
| $E$ | −844.9 | −852.9 | −855.9 | −857.5 | −858.5 | −859.2 | −862.8(7) |

DMRG yields two separate results: a variational upper bound and an extrapolated number based on the different bond dimensions. The lowest variational correlation energy is $\Delta E_{\mathrm{DMRG(var)}} = -859.5$ m$E_{\mathrm{H}}$, corresponding to the $M = 7000$ result from the partially converged forwards schedule. The linear extrapolation was based on using the fully converged backwards schedule results for $M = 6000$ to $M = 1000$ (the variational $M = 6000$ result was $-859.2$ m$E_{\mathrm{H}}$) giving a final number of $\Delta E_{\mathrm{DMRG}(\infty)} = -862.8$ m$E_{\mathrm{H}}$, cf. Figure S2. The standard practice in DMRG for estimating an error from the extrapolation is to report a fraction of the extrapolation distance, typically 1/5. Here, the estimate (1/5 extrapolation distance error metric) is 0.7 m$E_{\mathrm{H}}$. The error of the linear fit (std. dev. of the intercept) is

about 0.2 m$E_\mathrm{H}$, suggesting the 1/5 extrapolation distance error is an overestimate.

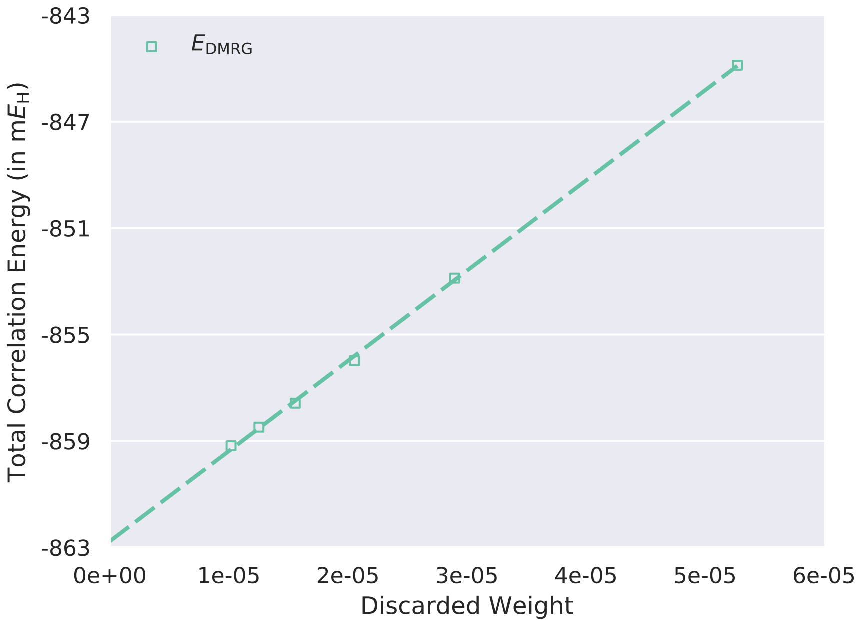


**Figure S2:** DMRG results.

## 5 AS-FCIQMC

For details on the adaptive shift formalism, please see Ref. S20. All AS-FCIQMC calculations were performed using the `NECI` code[S21,S22] in parallel on Intel Xeon CPU E5-2698v4 nodes (40 cores @ 2.2 GHz, 6.4 GB/core). The orbitals used were those of a preceding RHF calculation and the FCIQMC runs were performed in a basis of pure Slater determinants (no spin adaptation). Following an equilibration run with $1.0 \times 10^8$ walkers (yielding a correlation energy of $\Delta E_\mathrm{AS\text{-}FCIQMC(init)} = -863.3 \pm 0.9$ m$E_\mathrm{H}$), a first calculation with $1.0 \times 10^9$ (1B) walkers (growing from $1.0 \times 10^8$) yielded a correlation energy $\Delta E_\mathrm{AS\text{-}FCIQMC(1B)} = -864.8 \pm 0.5$ m$E_\mathrm{H}$. Next, a second calculation with $2.0 \times 10^9$ (2B) walkers (growing from $1.0 \times 10^9$) resulted in a correlation energy of $\Delta E_\mathrm{AS\text{-}FCIQMC(2B)} = -863.7 \pm 0.3$ m$E_\mathrm{H}$. The stochastic error bar of 0.3 m$E_\mathrm{H}$ is derived by averaging over the last 2637 time steps (discarding the first 5000 time steps for walker growth and equilibration period), and doing a blocking analysis.

The AS-FCIQMC(2B) result is used in Fig. 1 of the main text. For the largest AS-FCIQMC calculations (2B), the `NECI` code used 2.6 GB/core, i.e., 3162 Gb in total distributed over 32 nodes (40 cores/node).

# 6 CAD-FCIQMC

The CAD-FCIQMC approach, introduced in Ref. S23, belongs to a new category of semi-stochastic methods, in which information about higher-order wave function components extracted from the FCIQMC[S20,S24,S25] or CCMC[S26,S27] propagations is read into deterministic CC computations.[S23,S28–S30] CAD-FCIQMC can also be classified as an externally corrected CC method.[S31–S39] We recall that all externally corrected CC approaches are based on the observation that as long as the Hamiltonian does not contain higher–than–two-body interactions, the CC amplitude equations projected on the singly and doubly excited determinants, in which no approximations are made, do not engage higher–than–four-body components of the cluster operator $T$. Thus, by solving these equations for the singly and doubly excited clusters, $T_1$ and $T_2$, respectively, in the presence of their exact triply ($T_3$) and quadruply ($T_4$) excited counterparts extracted from FCI, one obtains the exact $T_1$ and $T_2$ and the exact correlation energy, which is given by the expression

$$\Delta E = \langle \Phi | \left[ H_N \exp(T_1 + T_2) \right]_C | \Phi \rangle, \tag{S1}$$

where $H_N = H - \langle \Phi | H | \Phi \rangle$ is the Hamiltonian in the normal-ordered form relative to the reference determinant $|\Phi\rangle$ and the subscript $C$ designates the connected operator product. This means that by using a well-behaved source of the $T_3$ and $T_4$ clusters, capable of offering their accurate description for the $N$-electron system of interest, one can obtain highly accurate $T_1$, $T_2$, and $\Delta E$. In the case of CAD-FCIQMC, this well-behaved source is the FCIQMC wave function $|\Psi^{(\mathrm{MC})}(\tau)\rangle$ obtained at a sufficiently long propagation time $\tau$, which converges to the corresponding FCI ground state as $\tau$ approaches $\infty$.

In order to extract the desired triply and quadruply excited clusters from the FCIQMC state $|\Psi^{(\mathrm{MC})}(\tau)\rangle$, we rewrite it to satisfy the intermediate normalization as

$$|\Psi^{(\mathrm{MC})}(\tau)\rangle = [1 + C^{(\mathrm{MC})}(\tau)]|\Phi\rangle \equiv \left[1 + \sum_{n=1}^{N} C_n^{(\mathrm{MC})}(\tau)\right]|\Phi\rangle, \tag{S2}$$

where $C_n^{(\mathrm{MC})}(\tau)$ are the CI excitation operators determined by counting walkers at the $n$-tuply excited determinants contributing to $|\Psi^{(\mathrm{MC})}(\tau)\rangle$ (dividing the numbers of these walkers by the number of walkers at $|\Phi\rangle$), replace Eq. (S2) by the equivalent exponential ansatz,

$$|\Psi^{(\mathrm{MC})}(\tau)\rangle = \exp[T^{(\mathrm{MC})}(\tau)]|\Phi\rangle \equiv \exp\left[\sum_{n=1}^{N} T_n^{(\mathrm{MC})}(\tau)\right]|\Phi\rangle, \tag{S3}$$

where $T^{(\mathrm{MC})}(\tau)$ is defined as $\ln[1+C^{(\mathrm{MC})}(\tau)]$, and exploit the resulting relationships between the CI excitation operators $C_n^{(\mathrm{MC})}(\tau)$ and their CC counterparts $T_n^{(\mathrm{MC})}(\tau)$ (see Ref. S23). Assuming that $|\Psi^{(\mathrm{MC})}(\tau)\rangle$ converges to the FCI wave function as $\tau$ increases, by solving the CC amplitude equations projected on the singly and doubly excited determinants, $|\Phi_i^a\rangle$ and $|\Phi_{ij}^{ab}\rangle$, respectively, in which $T_3$ and $T_4$ are replaced by their $T_3^{(\mathrm{MC})}(\tau)$ and $T_4^{(\mathrm{MC})}(\tau)$ counterparts obtained from the cluster analysis of $|\Psi^{(\mathrm{MC})}(\tau)\rangle$, i.e.,

$$\begin{aligned} \langle\Phi_i^a|\left[H_N \exp(T_1 + T_2 + T_3^{(\mathrm{MC})}(\tau))\right]_C|\Phi\rangle &= 0, \\ \langle\Phi_{ij}^{ab}|\left[H_N \exp(T_1 + T_2 + T_3^{(\mathrm{MC})}(\tau) + T_4^{(\mathrm{MC})}(\tau))\right]_C|\Phi\rangle &= 0, \end{aligned} \tag{S4}$$

for the singly and doubly excited clusters $T_1$ and $T_2$, we are guaranteed to obtain the exact $T_1$ and $T_2$ and thus the exact, FCI, correlation energy in the $\tau = \infty$ limit. In other words, if the walker population and propagation time $\tau$ used to generate the FCIQMC state $|\Psi^{(\mathrm{MC})}(\tau)\rangle$ are large enough, so that $T_3^{(\mathrm{MC})}(\tau)$ and $T_4^{(\mathrm{MC})}(\tau)$ extracted from $|\Psi^{(\mathrm{MC})}(\tau)\rangle$ and $T_1$ and $T_2$ obtained by solving the CC system defined by Eq. (S4) are good approximations to their exact, FCI or FCC, values, the CAD-FCIQMC correlation energy calculated using Eq. (S1) is anticipated to be a very accurate approximation to its FCI counterpart. The numerical

evidence reported in Ref. S23 shows that this is indeed the case. It is worth noting that one does not have to process the entire FCIQMC wave function $|\Psi^{(\mathrm{MC})}(\tau)\rangle$ to determine $T_3^{(\mathrm{MC})}(\tau)$ and $T_4^{(\mathrm{MC})}(\tau)$ entering Eq. (S4); all one needs to know are the CI excitation amplitudes through quadruples defining the $C_n^{(\mathrm{MC})}(\tau)$ operators with $n = 1$–4.

As shown in Ref. S23, by considering the CC system given by Eq. (S4) and by solving it for $T_1$ and $T_2$ deterministically, the CAD-FCIQMC approach can substantially accelerate the purely stochastic FCIQMC calculations. It also offers an interesting diagnostic of the quality of the instantaneous FCIQMC wave function $|\Psi^{(\mathrm{MC})}(\tau)\rangle$ obtained at a given time $\tau$, especially of its $C_n^{(\mathrm{MC})}(\tau)$ components through $n = 4$, using computational steps that are similar to those characterizing the conventional CCSD method[S40] once the cluster analysis of $|\Psi^{(\mathrm{MC})}(\tau)\rangle$, needed to determine $T_3^{(\mathrm{MC})}(\tau)$ and $T_4^{(\mathrm{MC})}(\tau)$, is completed. The latter feature is particularly useful in the context of the present study. Indeed, if in the process of solving the CC amplitude equations defined by Eq. (S4) the $T_1$ and $T_2$ clusters significantly relax compared to their initial $T_1^{(\mathrm{MC})}(\tau)$ and $T_2^{(\mathrm{MC})}(\tau)$ values extracted from $|\Psi^{(\mathrm{MC})}(\tau)\rangle$, so that the final CAD-FCIQMC correlation energy $\Delta E$, calculated using Eq. (S1), is considerably different than its instantaneous FCIQMC counterpart determined at time $\tau$,

$$\begin{aligned}\Delta E^{(\mathrm{MC})} &= \langle\Phi|H_N\left[C_1^{(\mathrm{MC})}(\tau)+C_2^{(\mathrm{MC})}(\tau)\right]|\Phi\rangle \\ &= \langle\Phi|\left[H_N\exp(T_1^{(\mathrm{MC})}(\tau)+T_2^{(\mathrm{MC})}(\tau))\right]_C|\Phi\rangle,\end{aligned} \tag{S5}$$

we can conclude that the FCIQMC wave function $|\Psi^{(\mathrm{MC})}(\tau)\rangle$ is not well converged yet. On the other hand, if $T_3^{(\mathrm{MC})}(\tau)$ and $T_4^{(\mathrm{MC})}(\tau)$ obtained by the cluster analysis of $|\Psi^{(\mathrm{MC})}(\tau)\rangle$ are nearly exact, $T_1$, $T_2$, and $\Delta E$ will relax very little during the CC iterations based on Eq. (S4) compared to their $T_1^{(\mathrm{MC})}(\tau)$, $T_2^{(\mathrm{MC})}(\tau)$, and $\Delta E^{(\mathrm{MC})}$ values. This means that if the final CAD-FCIQMC correlation energy $\Delta E$, Eq. (S1), obtained after solving the CC system defined by Eq. (S4), and its initial FCIQMC counterpart $\Delta E^{(\mathrm{MC})}$, Eq. (S5), agree to within a certain numerical precision, we may be able to claim that the CAD-FCIQMC estimate of the correlation energy is stable to within the same precision. This follows the observation,

which is a formal basis of all externally corrected CC approaches, that if $T_3^{(\mathrm{MC})}(\tau)$ and $T_4^{(\mathrm{MC})}(\tau)$ were exact, $T_1$ and $T_2$ obtained by solving Eq. (S4) would become exact too, i.e., the relaxation of $T_1$, $T_2$, and $\Delta E$ compared to their $T_1^{(\mathrm{MC})}(\tau)$, $T_2^{(\mathrm{MC})}(\tau)$, and $\Delta E^{(\mathrm{MC})}$ values would be zero.

The deterministic *a posteriori* CAD-FCIQMC steps, as summarized above, may provide useful insights into the error bounds associated with the FCIQMC wave functions, but this is not to say that these steps alone provide complete information about errors. In analyzing the results of CAD-FCIQMC calculations, we have to keep in mind that the underlying FCIQMC wave function propagations have their own intrinsic errors, which the deterministic CAD-FCIQMC steps cannot eliminate, such as the errors resulting from the use of the initiator algorithm and finite walker population. This means that CAD-FCIQMC can provide us with accurate estimates of the $\tau = \infty$ limit of a given FCIQMC propagation, without having to go through time-consuming equilibration and blocking analysis, but it cannot eliminate errors resulting from the use of finite walker populations in determining the FCIQMC wave functions. Furthermore, there exist special cases of external wave functions serving as sources of $T_3$ and $T_4$ clusters in the CC amplitude equations for $T_1$ and $T_2$ of the type of Eq. (S4), namely, all CC states defined by $T = \sum_{n=1}^{M} T_n$ with $M \geq 4$, starting from CCSDTQ,[S41,S42] where errors determined through the above amplitude and correlation energy relaxation argument are by definition zero, even though the CC states with $M < N$ are not exact. On the other hand, it is unlikely that any of the FCIQMC wave functions $|\Psi^{(\mathrm{MC})}(\tau)\rangle$, which are obtained in stochastic processes allowing walkers to explore the entire $N$-electron Hilbert space without setting up *a priori* constraints regarding the cluster structure of $|\Psi^{(\mathrm{MC})}(\tau)\rangle$, is a CC state with $T = \sum_{n=1}^{M} T_n$ and $4 \leq M < N$. Thus, the degree of relaxation of the singly and doubly excited clusters and correlation energy, resulting from solving Eq. (S4) for $T_1$ and $T_2$ in the presence of $T_3^{(\mathrm{MC})}(\tau)$ and $T_4^{(\mathrm{MC})}(\tau)$ extracted from the FCIQMC state $|\Psi^{(\mathrm{MC})}(\tau)\rangle$, compared to their $T_1^{(\mathrm{MC})}(\tau)$, $T_2^{(\mathrm{MC})}(\tau)$, and $\Delta E^{(\mathrm{MC})}$ values, combined with the changes in the final CAD-FCIQMC correlation energy $\Delta E$ as a consequence of increasing

the propagation time $\tau$, as in Ref. S23, or, as has been done in this work, where $\tau$s were sufficiently long, as a consequence of increasing the target walker population in the AS-FCIQMC algorithm discussed in Section 5, provides us with trustworthy estimates of the accuracy of CAD-FCIQMC computations. We will rely on these estimates when discussing the CAD-FCIQMC results for benzene summarized in Table S5 in a later part of this section.

Following the above description, the CAD-FCIQMC algorithm consists of the following three steps:[S23] **(i)** a stochastic FCIQMC run to produce the wave function $|\Psi^{(\mathrm{MC})}(\tau)\rangle$ for the subsequent cluster analysis (it is sufficient to store the CI excitation amplitudes through $C_4^{(\mathrm{MC})}(\tau)$), **(ii)** a cluster analysis of $|\Psi^{(\mathrm{MC})}(\tau)\rangle$ to extract the $T_n^{(\mathrm{MC})}(\tau)$ components with $n = 1$–$4$ from the corresponding $C_n^{(\mathrm{MC})}(\tau)$ amplitudes, and **(iii)** a deterministic CCSD-like calculation using Eq. (S4) in which one solves for the $T_1$ and $T_2$ clusters in the presence of the $T_3^{(\mathrm{MC})}(\tau)$ and $T_4^{(\mathrm{MC})}(\tau)$ components extracted from $|\Psi^{(\mathrm{MC})}(\tau)\rangle$. In the case of the CAD-FCIQMC calculations for the benzene/cc-pVDZ system reported in this work, summarized in Table S5 (see, also, Table S2 and Fig. 1 in the main text), the underlying FCIQMC computations defining step (i), which were performed using the `NECI` code,[S21] exploited the AS-FCIQMC algorithm developed in Ref. S20. The details of these calculations can be found in Section 5. Here, we only mention that the following instantaneous FCIQMC wave functions $|\Psi^{(\mathrm{MC})}(\tau)\rangle$ were subjected to CAD-FCIQMC processing: the AS-FCIQMC state obtained at the end of the equilibration period defined by 1 billion (1B) walkers, which we abbreviate as $|\Psi_{\mathrm{1B}}^{(\text{AS-FCIQMC})}\rangle$, and the AS-FCIQMC state, abbreviated as $|\Psi_{\mathrm{2B}}^{(\text{AS-FCIQMC})}\rangle$, obtained at the end of the equilibration period defined by 2 billion (2B) walkers. To test the numerical stability of our highest-level CAD-FCIQMC results using 2B walkers, we also attempted to replace the instantaneous $|\Psi_{\mathrm{2B}}^{(\text{AS-FCIQMC})}\rangle$ wave function by the AS-FCIQMC(2B) state obtained by averaging the last 100 time steps, which we abbreviate as $|\Psi_{\mathrm{2B}}^{(\text{AS-FCIQMC})}(\text{100-avg})\rangle$.

Once the $|\Psi_{\mathrm{1B}}^{(\text{AS-FCIQMC})}\rangle$, $|\Psi_{\mathrm{2B}}^{(\text{AS-FCIQMC})}\rangle$, and $|\Psi_{\mathrm{2B}}^{(\text{AS-FCIQMC})}(\text{100-avg})\rangle$ states were generated and the required CI excitation amplitudes through $C_4^{(\mathrm{MC})}(\tau)$ were stored, the re-

maining deterministic steps of the CAD-FCIQMC procedure, including the cluster analysis of each of the above AS-FCIQMC wave functions (step (ii)) and the final CCSD-like calculations of $T_1$ and $T_2$ based on Eq. (S4) (step (iii)), were performed with the in-house codes developed by the Piecuch group in this project, which were interfaced with `NECI` and which used the same sets of one- and two-electron molecular integrals (corresponding to the RHF basis) as those employed in the underlying AS-FCIQMC calculations. These codes are characterized by several improvements compared to our initial implementation of the CAD-FCIQMC approach reported in Ref. S23, which required storing the $T_3^{(\mathrm{MC})}(\tau)$ and $T_4^{(\mathrm{MC})}(\tau)$ vectors prior to constructing the CC amplitude equations defined by Eq. (S4). The CAD-FCIQMC codes used in this work eliminate the need for storing large sets of $T_4^{(\mathrm{MC})}(\tau)$ cluster amplitudes, such as those that correspond to the $|\Psi_{1\mathrm{B}}^{(\text{AS-FCIQMC})}\rangle$, $|\Psi_{2\mathrm{B}}^{(\text{AS-FCIQMC})}\rangle$, and $|\Psi_{2\mathrm{B}}^{(\text{AS-FCIQMC})}(100\text{-avg})\rangle$ wave functions for benzene. They store the $T_1^{(\mathrm{MC})}(\tau)$, $T_2^{(\mathrm{MC})}(\tau)$, and $T_3^{(\mathrm{MC})}(\tau)$ vectors extracted from the underlying AS-FCIQMC wave functions prior to constructing the CC amplitude equations for $T_1$ and $T_2$ defined by Eq. (S4), while processing the $T_4^{(\mathrm{MC})}(\tau)$ amplitudes produced during the cluster analysis steps on the fly, saving only the $T_4^{(\mathrm{MC})}(\tau)$-containing $\langle\Phi_{ij}^{ab}|[H_N T_4^{(\mathrm{MC})}(\tau)]_C|\Phi\rangle$ contributions to Eq. (S4), whose number equals the number of the doubly excited determinants $|\Phi_{ij}^{ab}\rangle$. In principle, we could also avoid storing the $T_3^{(\mathrm{MC})}(\tau)$ vectors, which would be particularly easy to do in the case of the linear $\langle\Phi_i^a|[H_N T_3^{(\mathrm{MC})}(\tau)]_C|\Phi\rangle$ and $\langle\Phi_{ij}^{ab}|[H_N T_3^{(\mathrm{MC})}(\tau)]_C|\Phi\rangle$ contributions, but we have not done it yet, since the third $T_3^{(\mathrm{MC})}(\tau)$-containing term in the CC system defined by Eq. (S4), namely, $\langle\Phi_{ij}^{ab}|[H_N T_1 T_3^{(\mathrm{MC})}(\tau)]_C|\Phi\rangle$, in which $T_3^{(\mathrm{MC})}(\tau)$ is fixed at its FCIQMC value and $T_1$ is iterated, would require additional changes in the CC routines used to set up Eq. (S4) in this work, which are beyond the scope of the present study. It is worth pointing out though that unlike $T_4^{(\mathrm{MC})}(\tau)$, which becomes quickly unmanageable as the system size increases, the $T_3^{(\mathrm{MC})}(\tau)$ amplitude vector is not difficult to store for the molecules of the size of benzene. Formally, $T_3^{(\mathrm{MC})}(\tau)$ is a three-body component of $T$, suggesting large computational costs, but by the virtue of a stochastic wave function sampling during FCIQMC propaga-

tions the numbers of nonzero amplitudes in the $T_3^{(\mathrm{MC})}(\tau)$ vectors are much smaller than the numbers of all triples in the corresponding $T_3$ operators. Thus, storing $T_3^{(\mathrm{MC})}(\tau)$ prior to constructing the $T_3^{(\mathrm{MC})}(\tau)$-containing terms in Eq. (S4) is not a major bottleneck, when medium-size systems, such as benzene, are examined. Storing $T_4^{(\mathrm{MC})}(\tau)$ is, so pre-computing the $\langle \Phi_{ij}^{ab} | [H_N T_4^{(\mathrm{MC})}(\tau)]_C | \Phi \rangle$ contributions to Eq. (S4) during the cluster analysis is a lot more important.

As a result of the above improvements in our CAD-FCIQMC codes, both the cluster analyses of the AS-FCIQMC wave functions (to be precise, of the CI excitation amplitudes through quadruples defining these wave functions) and the final CC iterations based on Eq. (S4) represented a relatively inexpensive computational effort when the benzene/cc-pVDZ system was examined. Indeed, the cluster analysis of the one-billion-walker state $|\Psi_{1\mathrm{B}}^{(\text{AS-FCIQMC})}\rangle$ required 5.6 hours using a single core of a shared-memory (SMP) node from Dell consisting of two 10-core Intel Xeon Silver 4114 2.20 GHz processors with 25.6 GB memory per core. In the case of the two-billion-walker states $|\Psi_{2\mathrm{B}}^{(\text{AS-FCIQMC})}\rangle$ and $|\Psi_{2\mathrm{B}}^{(\text{AS-FCIQMC})}(\text{100-avg})\rangle$, we needed 8.1 hours per state on the same machine to complete the cluster analysis step, again using only one core. The final CC iterations, in which we solved for the $T_1$ and $T_2$ clusters in the presence of the $T_3^{(\mathrm{MC})}(\tau)$ and $T_4^{(\mathrm{MC})}(\tau)$ components extracted from the above AS-FCIQMC wave functions, required about 200 seconds on all 20 cores of the aforementioned Dell node to reach convergence. We typically needed 10 iterations to converge the CAD-FCIQMC energies to within $10^{-6}\, E_{\mathrm{H}}$ when using the $T_1^{(\mathrm{MC})}(\tau)$ and $T_2^{(\mathrm{MC})}(\tau)$ amplitudes extracted from the AS-FCIQMC wave functions as initial guesses for $T_1$ and $T_2$ in the CCSD-like calculations based on Eq. (S4).

The disk storage and memory requirements characterizing the CAD-FCIQMC calculations for the benzene/cc-pVDZ system considered in this study were relatively modest too. We illustrate them by the most demanding CAD-FCIQMC runs based on processing the two-billion-walker AS-FCIQMC states, such as $|\Psi_{2\mathrm{B}}^{(\text{AS-FCIQMC})}\rangle$. The `NECI` output file containing the $|\Psi_{2\mathrm{B}}^{(\text{AS-FCIQMC})}\rangle$ wave function up to $C_4^{(\mathrm{MC})}(\tau)$ contributions was about 49 GB

in size. About 35 GB of this were the data used in the cluster analysis (the list of determinants through quadruples contributing to $|\Psi_{2B}^{(\text{AS-FCIQMC})}\rangle$ along with the corresponding walker numbers), and the rest was the information relevant to the AS-FCIQMC run that produced $|\Psi_{2B}^{(\text{AS-FCIQMC})}\rangle$ which we did not need and could discard. As already explained, the $T_4^{(\text{MC})}(\tau)$ amplitudes extracted from the AS-FCIQMC wave functions used in the CAD-FCIQMC calculations reported in this work, needed to construct the $\langle\Phi_{ij}^{ab}|[H_N T_4^{(\text{MC})}(\tau)]_C|\Phi\rangle$ contributions to Eq. (S4), were processed on the fly, so we did not have to store them, but the $T_1^{(\text{MC})}(\tau)$, $T_2^{(\text{MC})}(\tau)$, and $T_3^{(\text{MC})}(\tau)$ vectors produced during the cluster analysis were saved. For each of the AS-FCIQMC states considered in this study, we saved them as a single disk file. To facilitate and speed up the cluster analysis and the subsequent CC calculations based on Eq. (S4), we kept all of the $T_2^{(\text{MC})}(\tau)$ and $T_3^{(\text{MC})}(\tau)$ amplitudes, including those obtained by permuting orbital indices, i.e., not just the non-redundant ones, in that file. As a result, for the most demanding, two-billion-walker AS-FCIQMC states considered in this work, such as $|\Psi_{2B}^{(\text{AS-FCIQMC})}\rangle$, the file containing the $T_1^{(\text{MC})}(\tau)$, $T_2^{(\text{MC})}(\tau)$, and $T_3^{(\text{MC})}(\tau)$ amplitudes was about 81 GB in size. Given the fact that the aforementioned SMP Dell node used in the deterministic steps of our CAD-FCIQMC calculations had a sufficiently large memory (512 GB total), during each of the cluster analyses performed in this work we kept the file containing the AS-FCIQMC wave function information through quadruples and the file containing the $T_1^{(\text{MC})}(\tau)$, $T_2^{(\text{MC})}(\tau)$, and $T_3^{(\text{MC})}(\tau)$ amplitudes, as described above, in memory. This meant using 116 GB of resident memory during the cluster analysis of the most demanding, two-billion-walker AS-FCIQMC states considered in this work (35 GB for the wave function information through quadruples and 81 GB for the $T_1^{(\text{MC})}(\tau)$, $T_2^{(\text{MC})}(\tau)$, and $T_3^{(\text{MC})}(\tau)$ amplitudes). We kept the $T_1^{(\text{MC})}(\tau)$, $T_2^{(\text{MC})}(\tau)$, and $T_3^{(\text{MC})}(\tau)$ amplitudes (81 GB), along with the $T_1$ and $T_2$ vectors and the relevant intermediates needed to construct the CC equations based on Eq. (S4) ($< 1$ GB), in memory as well.

The CAD-FCIQMC results for the benzene/cc-pVDZ system considered in this study are summarized in Table S5. Following the above description, and to facilitate our error

**Table S5:** Results of the CAD-FCIQMC calculations based on the AS-FCIQMC wave functions obtained after equilibration runs using 1 billion (1B) and 2 billion (2B) walkers.

| Calculation | $\Delta E/\text{m}E_\text{H}$ |
|---|---|
| AS-FCIQMC(1B) | $-864.8 \pm 0.5$ |
| CAD-FCIQMC-ext(1B) | $-867.010$ |
| CAD-FCIQMC[1–5](1B) | $-864.089$ |
| CAD-FCIQMC[1,(3+4)/2](1B) | $-863.861$ |
| AS-FCIQMC(2B) | $-863.7 \pm 0.3$ |
| CAD-FCIQMC-ext(2B) | $-863.464$ |
| CAD-FCIQMC[1–5](2B) | $-863.453$ |
| CAD-FCIQMC[1,(3+4)/2](2B) | $-863.438$ |
| CAD-FCIQMC-ext(2B,100-avg) | $-863.460$ |
| CAD-FCIQMC[1–5](2B,100-avg) | $-863.439$ |

analysis, along with the final CAD-FCIQMC correlation energies $\Delta E$, determined using Eq. (S1) after solving for the $T_1$ and $T_2$ clusters in the presence of $T_3^{(\text{MC})}(\tau)$ and $T_4^{(\text{MC})}(\tau)$ extracted from the AS-FCIQMC wave functions, abbreviated as CAD-FCIQMC[1–5] and CAD-FCIQMC[1,(3+4)/2], we show the initial projected correlation energies $\Delta E^{(\text{MC})}$, Eq. (S5), calculated using the $T_1^{(\text{MC})}(\tau)$ and $T_2^{(\text{MC})}(\tau)$ amplitudes prior to the CC iterations based on Eq. (S4), abbreviated as CAD-FCIQMC-ext. We also show the results of the underlying AS-FCIQMC propagations, along with the corresponding error bars, obtained after equilibrating walker populations and performing the blocking analyses discussed in Section 5. For clarity of our presentation, each of the acronyms seen in Table S5 is augmented with the information about the target walker population used in the stochastic AS-FCIQMC run preceding the deterministic CAD-FCIQMC steps. Thus, the CAD-FCIQMC-ext(1B), CAD-FCIQMC[1–5](1B), and CAD-FCIQMC[1,(3+4)/2](1B) correlation energies correspond to the instantaneous AS-FCIQMC(1B) state obtained at the end of the equilibration period using 1 billion walkers, which we previously abbreviated as $|\Psi_{1\text{B}}^{(\text{AS-FCIQMC})}\rangle$, whereas the CAD-FCIQMC-ext(2B), CAD-FCIQMC[1–5](2B), and CAD-FCIQMC[1,(3+4)/2](2B) results correspond to $|\Psi_{2\text{B}}^{(\text{AS-FCIQMC})}\rangle$. The last two correlation energies in Table S5, designated as CAD-FCIQMC-ext(2B,100-avg) and CAD-FCIQMC[1–5](2B,100-avg), correspond to the

two-billion-walker AS-FCIQMC(2B) state obtained by averaging the last 100 time steps, abbreviated as $|\Psi_{2B}^{(\text{AS-FCIQMC})}(100\text{-avg})\rangle$. The information in the square brackets at the CAD-FCIQMC acronyms in Table S5 indicates the $(T_2)^2$ Goldstone-Hugenholtz diagrams entering the CCSD-like system used in the final stage of the CAD-FCIQMC calculations (adopting the diagram numbering taken from Fig. 4 in Ref. S32) that were treated deterministically by solving the respective CC amplitude equations. Thus, CAD-FCIQMC[1–5] means that all five $(T_2)^2$ Goldstone-Hugenholtz diagrams of the CCSD-like system defined by Eq. (S4) were treated deterministically, whereas CAD-FCIQMC[1,(3+4)/2] implies that only diagram 1 and an average of diagrams 3 and 4, which are responsible for capturing strong correlations (originally considered in one of the approximate coupled-pair theories discovered and tested in Ref. S43, which was re-discovered as a distinguishable cluster approximation in Ref. S44), were evaluated using the $T_2$ amplitudes obtained by solving the CC equations, with the rest of $(T_2)^2$ calculated using $T_2^{(\text{MC})}(\tau)$ extracted from FCIQMC. Much of the discussion in this section focuses on the CAD-FCIQMC[1–5] approach, as introduced in Ref. S23. The CAD-FCIQMC[1,(3+4)/2] algorithm will be discussed in detail in a separate publication.[S45]

As shown in Table S5, there is a great deal of consistency among the CAD-FCIQMC results, especially when the two-billion walker $|\Psi_{2B}^{(\text{AS-FCIQMC})}\rangle$ and $|\Psi_{2B}^{(\text{AS-FCIQMC})}(100\text{-avg})\rangle$ states are used as sources of the triply and quadruply excited clusters. In this case, the relaxation of the $T_1$ and $T_2$ clusters and correlation energy $\Delta E$, resulting from iterating $T_1$ and $T_2$ in the presence of $T_3^{(\text{MC})}(\tau)$ and $T_4^{(\text{MC})}(\tau)$ extracted from $|\Psi_{2B}^{(\text{AS-FCIQMC})}\rangle$ and $|\Psi_{2B}^{(\text{AS-FCIQMC})}(100\text{-avg})\rangle$, compared to the initial $T_1^{(\text{MC})}(\tau)$, $T_2^{(\text{MC})}(\tau)$, and $\Delta E^{(\text{MC})}$ values is virtually none, on the order of 0.01–0.03 m$E_{\text{H}}$ when the correlation energies are examined (cf. the CAD-FCIQMC[1–5](2B) and CAD-FCIQMC[1,(3+4)/2](2B) $\Delta E$ values in Table S5 with their CAD-FCIQMC-ext(2B) counterpart or CAD-FCIQMC[1–5](2B,100-avg) with CAD-FCIQMC-ext(2B,100-avg)). This suggests that the $|\Psi_{2B}^{(\text{AS-FCIQMC})}\rangle$ and $|\Psi_{2B}^{(\text{AS-FCIQMC})}(100\text{-avg})\rangle$ wave functions obtained in the AS-FCIQMC(2B) propagations using 2 billion walkers, at least their $C_n^{(\text{MC})}(\tau)$ components through $n = 4$, are numerically stable

and very well converged. Given the fact that the AS-FCIQMC propagations are allowed to explore the entire many-electron Hilbert space and populate determinants higher than quadruples, we can anticipate that the $C_n^{(\mathrm{MC})}(\tau)$ wave function components with $n > 4$, which are intrinsically coupled to their $n \leq 4$ counterparts during the AS-FCIQMC calculations, are accurately represented by $|\Psi_{2\mathrm{B}}^{(\text{AS-FCIQMC})}\rangle$ and $|\Psi_{2\mathrm{B}}^{(\text{AS-FCIQMC})}(100\text{-avg})\rangle$ as well. While, as pointed out above, the relaxation of $T_1$, $T_2$, and $\Delta E$ in the CC iterations based on Eq. (S4) could also become small if $|\Psi_{2\mathrm{B}}^{(\text{AS-FCIQMC})}\rangle$ and $|\Psi_{2\mathrm{B}}^{(\text{AS-FCIQMC})}(100\text{-avg})\rangle$ mimicked one of the truncated CC states with $T = \sum_{n=1}^{M} T_n$ and $4 \leq M < N$, we do not think that this is likely in the purely stochastic AS-FCIQMC runs that do not constrain the wave function's cluster structure. For example, neither $|\Psi_{2\mathrm{B}}^{(\text{AS-FCIQMC})}\rangle$ nor $|\Psi_{2\mathrm{B}}^{(\text{AS-FCIQMC})}(100\text{-avg})\rangle$ represent the CCSDTQ ($M = 4$) wave function or an approximation to it, since all of the CAD-FCIQMC correlation energies resulting from the use of $|\Psi_{2\mathrm{B}}^{(\text{AS-FCIQMC})}\rangle$ and $|\Psi_{2\mathrm{B}}^{(\text{AS-FCIQMC})}(100\text{-avg})\rangle$ differ from the CCSDTQ correlation energy by 1 m$E_{\mathrm{H}}$ or more. The remarkable numerical stability of the CAD-FCIQMC calculations using the two-billion-walker AS-FCIQMC states can be appreciated even more if we compare the CAD-FCIQMC[1–5](2B), CAD-FCIQMC[1,(3+4)/2](2B), and CAD-FCIQMC[1–5](2B,100-avg) correlation energies with one another. The CAD-FCIQMC[1–5](2B) and CAD-FCIQMC[1,(3+4)/2](2B) $\Delta E$ values agree to within 0.015 m$E_{\mathrm{H}}$, although some $(T_2)^2$ diagrams participating in the CC iterations defining the latter calculation were determined using the fixed $T_2^{(\mathrm{MC})}(\tau)$ amplitudes extracted from the $|\Psi_{2\mathrm{B}}^{(\text{AS-FCIQMC})}\rangle$ state. The CAD-FCIQMC[1–5](2B) and CAD-FCIQMC[1–5](2B,100-avg) correlation energies agree to within 0.014 m$E_{\mathrm{H}}$, although the former calculation uses the instantaneous $|\Psi_{2\mathrm{B}}^{(\text{AS-FCIQMC})}\rangle$ wave function obtained at the end of the equilibration period to determine $T_3^{(\mathrm{MC})}(\tau)$ and $T_4^{(\mathrm{MC})}(\tau)$, whereas the latter one relies on the $|\Psi_{2\mathrm{B}}^{(\text{AS-FCIQMC})}(100\text{-avg})\rangle$ state obtained by averaging the last 100 time steps during walker equilibration stage.

Our highest-level CAD-FCIQMC calculations using the two-billion-walker AS-FCIQMC states to provide the information about the triply and quadruply excited clusters suggest

that the FCI correlation energy for the benzene/cc-pVDZ system examined in this work can be estimated at $-863.44(1)\,\mathrm{m}E_{\mathrm{H}}$ (rounded up in Table S2 to $-863.4\,\mathrm{m}E_{\mathrm{H}}$). This result seems to be well converged in its own right, but it is additionally reassuring that all of our CAD-FCIQMC(2B) calculations, including those in which the $T_1$ and $T_2$ clusters were allowed to relax during the final CC iterations, fall within the error bars of the underlying AS-FCIQMC(2B) propagation, estimated at $\pm 0.3\,\mathrm{m}E_{\mathrm{H}}$, which were obtained completely independently after equilibrating walker populations and performing the blocking analysis involving the last 2,637 time steps, discussed in Section 5. In fact, there is a great deal of consistency between our CAD-FCIQMC[1–5](1B) and CAD-FCIQMC[1,(3+4)/2](1B) calculations, in which the $T_1$ and $T_2$ clusters were iterated in the presence of $T_3^{(\mathrm{MC})}(\tau)$ and $T_4^{(\mathrm{MC})}(\tau)$ extracted from the one-billion-walker $|\Psi_{\mathrm{1B}}^{(\mathrm{AS\text{-}FCIQMC})}\rangle$ state, and the purely stochastic AS-FCIQMC(1B) run. The correlation energy resulting from the CAD-FCIQMC calculations using $|\Psi_{\mathrm{1B}}^{(\mathrm{AS\text{-}FCIQMC})}\rangle$, obtained by averaging the CAD-FCIQMC[1–5](1B) and CAD-FCIQMC[1,(3+4)/2](1B) $\Delta E$ values, of $-864.0(1)\,\mathrm{m}E_{\mathrm{H}}$, is slightly outside the $\pm 0.5\,\mathrm{m}E_{\mathrm{H}}$ error bars of the underlying AS-FCIQMC(1B) propagation, but only slightly. In fact, the one-billion-walker AS-FCIQMC calculation is not as well converged as the AS-FCIQMC(2B) run, as can be seen by comparing the projected CAD-FCIQMC-ext(1B) correlation energy, calculated using the $T_1^{(\mathrm{MC})}(\tau)$ and $T_2^{(\mathrm{MC})}(\tau)$ amplitudes extracted from $|\Psi_{\mathrm{1B}}^{(\mathrm{AS\text{-}FCIQMC})}\rangle$, with the converged CAD-FCIQMC[1–5](1B) and CAD-FCIQMC[1,(3+4)/2](1B) $\Delta E$ values obtained after iterating $T_1$ and $T_2$. For example, the difference between the CAD-FCIQMC-ext(1B) correlation energy and its relaxed CAD-FCIQMC[1–5](1B) and CAD-FCIQMC[1,(3+4)/2](1B) counterparts is about $3\,\mathrm{m}E_{\mathrm{H}}$, as opposed to 0.02–0.03 $\mathrm{m}E_{\mathrm{H}}$ when we compare the analogous two-billion-walker data. Despite all this, our converged CAD-FCIQMC calculations utilizing $T_3^{(\mathrm{MC})}(\tau)$ and $T_4^{(\mathrm{MC})}(\tau)$ extracted from the $|\Psi_{\mathrm{1B}}^{(\mathrm{AS\text{-}FCIQMC})}\rangle$ state produce the correlation energy which is in good agreement with both the extrapolated AS-FCIQMC(1B) and AS-FCIQMC(2B) values and with our highest-level CAD-FCIQMC results obtained using the two-billion-walker AS-FCIQMC states. This illustrates the abil-

ity of the deterministic CC iterations used by the CAD-FCIQMC approach, in which we relax the $T_1$ and $T_2$ amplitudes in the presence of the triply and quadruply excited clusters extracted from FCIQMC, to accurately extrapolate the results of the long-time FCIQMC dynamics.

The fact that the substantial increase in the walker population in the underlying AS-FCIQMC calculations, from one to two billion, changes the final CAD-FCIQMC correlation energy very little is reassuring too, demonstrating that the semi-stochastic CAD-FCIQMC calculations are capable of reducing the walker population error of the underlying AS-FCIQMC propagations in a substantial manner. Indeed, the final CAD-FCIQMC correlation energies obtained by iterating $T_1$ and $T_2$ in the presence of $T_3^{(\mathrm{MC})}(\tau)$ and $T_4^{(\mathrm{MC})}(\tau)$ extracted from FCIQMC change only by about $0.5\,\mathrm{m}E_{\mathrm{H}}$ when the one-billion-walker $|\Psi_{1\mathrm{B}}^{(\text{AS-FCIQMC})}\rangle$ state is replaced by its two-billion-walker $|\Psi_{2\mathrm{B}}^{(\text{AS-FCIQMC})}\rangle$ and $|\Psi_{2\mathrm{B}}^{(\text{AS-FCIQMC})}(100\text{-avg})\rangle$ counterparts. This should be compared to the $1.1\,\mathrm{m}E_{\mathrm{H}}$ difference between the corresponding AS-FCIQMC(1B) and AS-FCIQMC(2B) correlation energies, although one should keep in mind that these energies carry stochastic errors estimated at $\pm 0.5\,\mathrm{m}E_{\mathrm{H}}$ and $\pm 0.3\,\mathrm{m}E_{\mathrm{H}}$, respectively. It is certainly encouraging that with a rather modest computational effort, the CAD-FCIQMC approach is capable of producing numerically stable and reasonably converged results. Given the above analysis and being conservative about the various errors that contribute to the CAD-FCIQMC calculations, we can conclude that our best FCI correlation energy estimate of about $-863.4\,\mathrm{m}E_{\mathrm{H}}$, which we use in the present study as our final CAD-FCIQMC value, is accurate to within $0.5\,\mathrm{m}E_{\mathrm{H}}$ (with the likelihood that the error bars associated with this result are even smaller).

# 7 SHCI

For details of the current version of SHCI theory, please see Refs. S46 and S47 as well as references therein. SHCI, in common with other selected configuration interaction plus per-

turbation theory (SCI+PT) methods, has two stages. In the first stage, a variational wave function is constructed iteratively, starting from a determinant that is expected to have a significant amplitude in the final wave function. The number of determinants in the variational wave function is controlled by a parameter $\epsilon_1$. In the second stage, second-order Epstein-Nesbet perturbation theory is used to improve upon the variational energy. The number of determinants used to compute the perturbative correction is controlled by a second parameter $\epsilon_2$, which is chosen in this study to be $\epsilon_2 = 10^{-3} \times \epsilon_1$. The total energy (sum of the variational energy and the perturbative correction) is computed at several values of $\epsilon_1$ and extrapolated to $\epsilon_1 \to 0$ to obtain an estimate for the FCI energy.

The convergence of the SHCI variational and total energies with respect to the number of determinants depends on the choice of orbitals. The simplest choice, Hartree-Fock orbitals, typically give slow convergence. Natural orbitals, obtained from SHCI, give faster convergence, and orbitals optimized within SHCI to minimize the variational energy at some fairly large value of $\epsilon_1$ give yet faster convergence. For molecules with more than a few atoms, split-localized optimized orbitals give faster convergence than delocalized optimized orbitals. In this study we used Pipek-Mezey split-localized optimized orbitals constructed using the methods described in Ref. S47. The value of $\epsilon_1$ used in the optimization was $2.0 \times 10^{-3}$ m$E_{\mathrm{H}}$ for the blind test, and $1.0 \times 10^{-4}$ m$E_{\mathrm{H}}$ for the subsequent improved calculations.

The final energy is obtained by a weighted fit of the total energies to a quadratic function of the perturbative correction, as shown in Fig. S4 for the calculation submitted for the blind test, and in Fig. S5 for the subsequent calculation that used better optimized orbitals and smaller values of $\epsilon_1$. The weight function used is the inverse square of the perturbative correction. Table S6 shows the same information in greater detail, including also the values of $\epsilon_1$ used and the number of time-reversal symmetrized determinants and the number of determinants. Our largest calculation included $5.4 \times 10^8$ determinants.

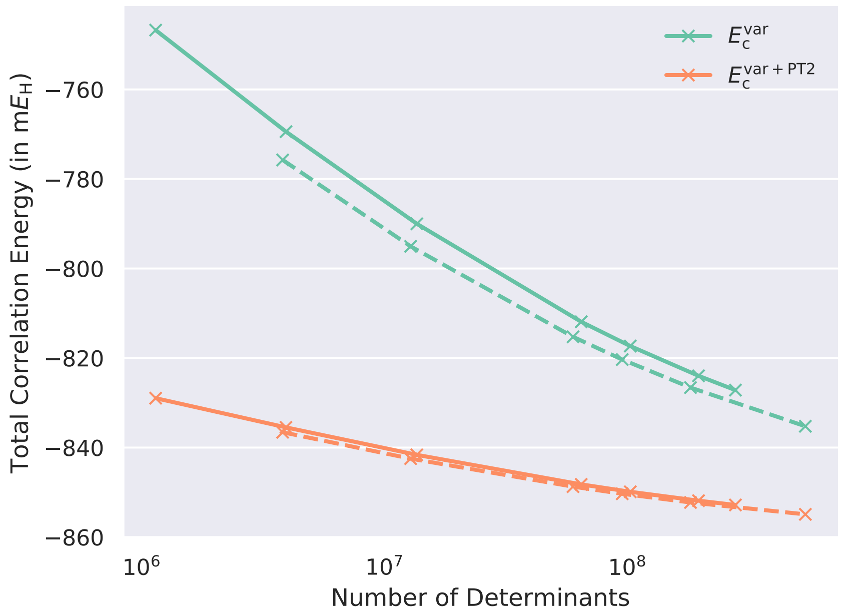


**Figure S3:** SHCI energies versus number of determinants. Blind test energies are plotted with solid lines, updated energies obtained with further optimized orbitals (not part of main study) are plotted with dashed lines.

The total energy provided for the blind test, −231.5861 $E_H$ was the value from the 7-point weighted quadratic fit shown in Table S6 along with a conservative estimate for the extrapolation error of 1.5 m$E_H$, which is almost an order of magnitude larger than the fit error. This corresponds to a correlation energy of −864.2 m$E_H$. In contrast to the statistical error, which has a well-defined probabilistic meaning, there is no well defined method for estimating the extrapolation error and different groups report wildly different estimates even when the underlying calculations are similar. In light of our subsequent calculations using better optimized orbitals and going down to smaller values of $\epsilon_1$, we could have gotten a slightly more accurate energy estimate of −231.5856 $E_H$ using the 5-point fit. Although the extrapolation curve is nearly linear, when sufficiently many data points are available, it is appropriate to perform a fit with a higher-order polynomial. The reduced chi-squared statistic can be used to avoid overfitting. A weighted cubic fit of either data set, using all the data points for that set, gives a total energy of −231.5851 $E_H$, corresponding to a

**Table S6:** SHCI variational and total energy convergence. The top block of the table is for the partially optimized orbitals used in the blind test, whereas the bottom block is for further optimized orbitals and smaller values of $\epsilon_1$. The errors in the total energies, $E_{\text{tot}}$, for finite values of $\epsilon_1$ are statistical errors. These are negligible, particularly for the smaller $\epsilon_1$ values. The errors in $E_{\text{tot}}$ extrapolated to $\epsilon_1 = 0$ are fit errors which typically greatly underestimate the actual extrapolation error. The energy reported in the blind test was that from the 7-point fit, with a conservative estimate of the extrapolation error which is almost an order of magnitude larger than the fit error.

| $\epsilon_1$ | $N_{\text{det}}^{\text{sym}}$ | $N_{\text{det}}$ | $E_{\text{var}}$ | $E_{\text{tot}}$ |
|---|---|---|---|---|
| $2.0 \times 10^{-4}$ | 579 708 | 1 134 081 | −231.468 564 | −231.550 787 ± 0.000 010 |
| $1.0 \times 10^{-4}$ | 1 975 676 | 3 901 848 | −231.491 252 | −231.557 309 ± 0.000 010 |
| $5.0 \times 10^{-5}$ | 6 790 526 | 13 486 304 | −231.511 826 | −231.563 444 ± 0.000 007 |
| $2.0 \times 10^{-5}$ | 32 178 640 | 64 100 382 | −231.533 720 | −231.570 044 ± 0.000 005 |
| $1.5 \times 10^{-5}$ | 51 218 692 | 102 088 555 | −231.539 142 | −231.571 697 ± 0.000 005 |
| $1.0 \times 10^{-5}$ | 97 754 454 | 194 977 798 | −231.545 790 | −231.573 686 ± 0.000 003 |
| $8.0 \times 10^{-6}$ | 138 641 259 | 276 617 654 | −231.548 984 | −231.574 641 ± 0.000 003 |
| Extrap. using 7 pts. | | | −231.586 064 | −231.586 064 ± 0.000 160 |
| Extrap. using 6 pts. | | | −231.585 772 | −231.585 772 ± 0.000 120 |
| Extrap. using 5 pts. | | | −231.585 569 | −231.585 569 ± 0.000 143 |
| $1.0 \times 10^{-4}$ | 1 914 692 | 3 780 337 | −231.497 568 | −231.558 399 ± 0.000 010 |
| $5.0 \times 10^{-5}$ | 6 410 037 | 12 722 141 | −231.516 872 | −231.564 290 ± 0.000 006 |
| $2.0 \times 10^{-5}$ | 29 787 396 | 59 310 339 | −231.537 074 | −231.570 545 ± 0.000 006 |
| $1.5 \times 10^{-5}$ | 47 463 030 | 94 569 745 | −231.542 155 | −231.572 140 ± 0.000 006 |
| $1.0 \times 10^{-5}$ | 90 601 302 | 180 662 587 | −231.548 415 | −231.574 081 ± 0.000 002 |
| $5.0 \times 10^{-6}$ | 268 931 930 | 536 792 289 | −231.557 059 | −231.576 736 ± 0.000 002 |
| Extrap. using 6 pts. | | | −231.585 609 | −231.585 609 ± 0.000 104 |
| Extrap. using 5 pts. | | | −231.585 464 | −231.585 464 ± 0.000 105 |

correlation energy of −863.3 m$E_{\text{H}}$. This should be considered to be the best post blind test SHCI estimate. Note that all the extrapolation estimates in this paragraph are well within the estimated error provided with the blind test.

All calculations were performed using the `Arrow` code.[S48] For the blind test runs, the calculations shown in Table S6 for $\epsilon_1 = 2.0 \times 10^{-4}$, $1.0 \times 10^{-4}$, $5.0 \times 10^{-5}$ and $2.0 \times 10^{-5}$ took in total 13 hours on four Intel(R) Xeon(R) Silver-4110 nodes (16 cores @ 2.1 GHz, 24 GB/core), and the calculations for $\epsilon_1 = 1.0 \times 10^{-5}$ and $8.0 \times 10^{-6}$ took in total 49 hours on

one Intel Xeon E7-8870v4 node (40 cores @ 2.1 GHz, 75 GB/core).

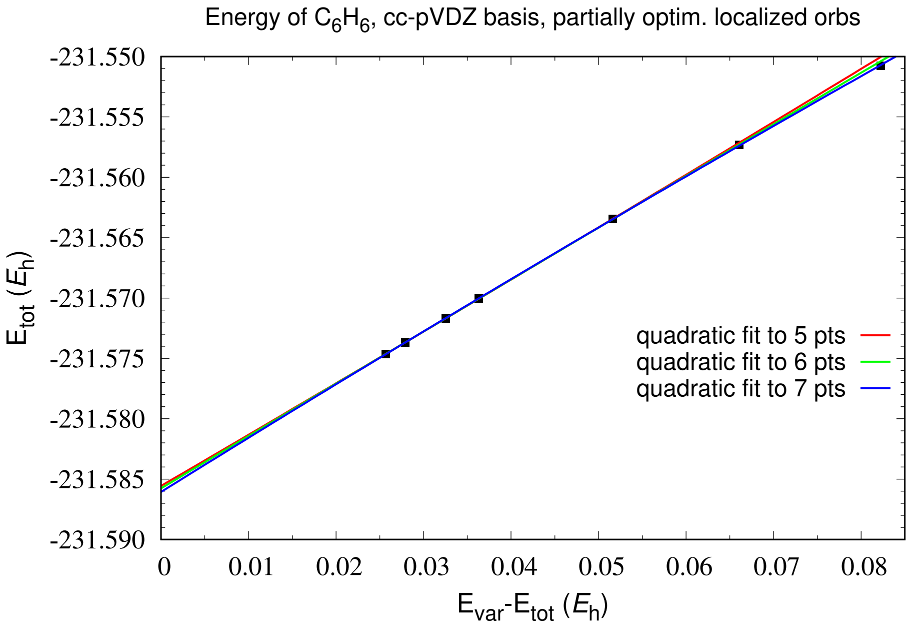


**Figure S4:** Convergence plot of SHCI total energies for the partially optimized orbitals used in the blind test. The lines are weighted quadratic fits, using varying number of points with the smallest $E_{\mathrm{var}} - E_{\mathrm{tot}}$ values.

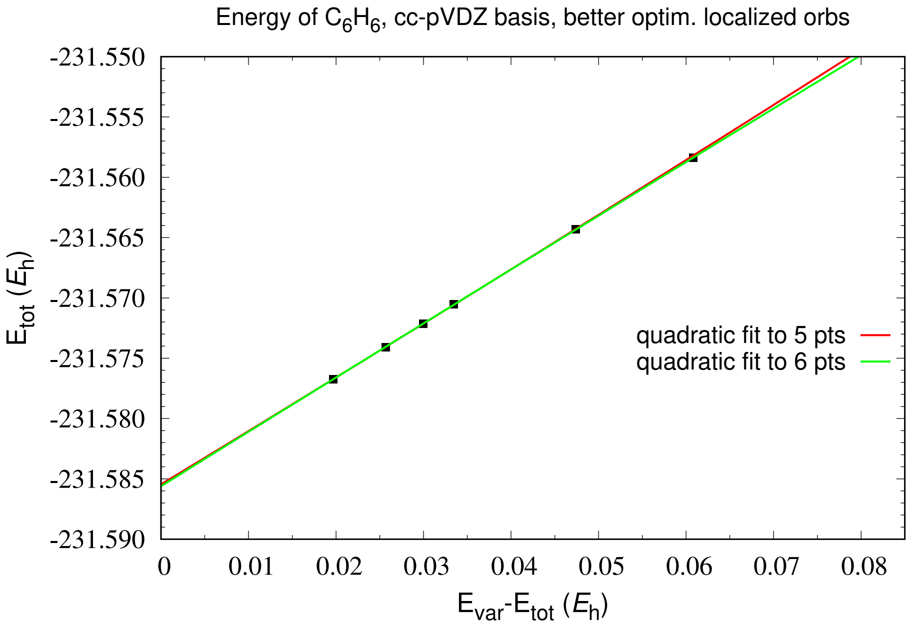


**Figure S5:** Convergence plot of SHCI total energies for further optimized orbitals and smaller $\epsilon_1$ values. The lines are weighted quadratic fits, using varying number of points with the smallest $E_{\mathrm{var}} - E_{\mathrm{tot}}$ values.

# 8 ASCI

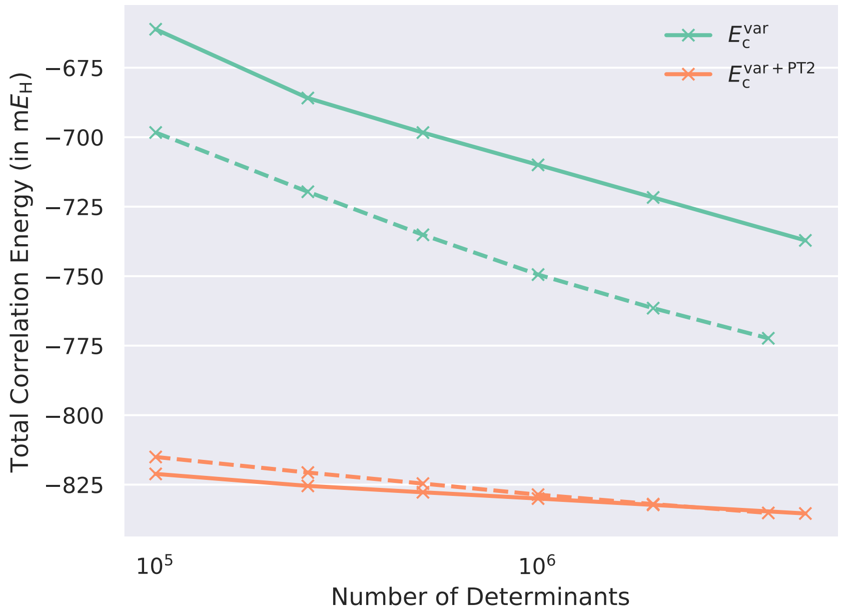


**Figure S6:** ASCI results. Original results are plotted with solid lines, updated localized orbital results (not part of main study) are plotted with dashed lines.

Details on the most recent version of ASCI theory has recently been presented elsewhere.[S49,S50] All ASCI calculations were performed using a development version of Q-Chem 5.2[S51] on AMD EPYC 7401 hardware (2.0 GHz, 5.3 GB/core). The CI component was run in parallel over 24 processors but the subsequent Epstein-Nesbet PT2 correction was computed on a single processor. The active space orbitals were optimized from canonical HF MOs in an multiconfigurational self-consistent field (MCSCF) manner (while only considering active-active rotations, i.e. keeping the core levels frozen), using $5 \times 10^5$ ASCI selected determinants,[S52] prior to PT2 calculations with varying number of determinants. The computed ASCI results are presented in Figure S6, and the final extrapolated correlation energy is estimated to be $\Delta E_{ASCI} = -860.0 \pm 0.2$ m$E_H$ with the error bar spanned by the uncertainty in the extrapolation towards the limit of zero PT2 correction (standard deviation of a linear fit with last 3 points, as described in Ref S53).

## 8.1 ASCI with localized orbitals

Subsequent to the blind challenge, an additional effort was made to determine the impact of using spatial symmetry broken localized orbitals as an initial guess instead of delocalized canonical MOs. The occupied canonical orbitals were consequently Pipek-Mezey localized[S7] and the virtual space subjected to the Sano procedure[S54] to obtain the corresponding antibonding orbitals. These resulting orbitals were similarly optimized by active-active rotations in an MCSCF manner, using $5 \times 10^5$ ASCI determinants.[S52] The optimized localized orbitals yielded significantly lower variational energies for a given size of ASCI wave function, although inclusion of PT2 resulted in values quite similar with those obtained from delocalized orbitals (as can be seen from Table S7 and Figure S6). The lower magnitude of PT2 corrections nonetheless suggest that the localized orbital ASCI values are more reliable, especially with respect to extrapolation (by virtue of being closer to the $E_{PT2} \rightarrow 0$ limit). Extrapolation of the results obtained using localized orbitals to $E_{PT2} \rightarrow 0$ limit yields a correlation energy of $-861.3 \pm 0.5$ m$E_{\mathrm{H}}$.

It is however worth noting that this localized orbital result is essentially outside the range estimated from the original delocalized case (-860.0 $\pm$ 0.2 m$E_{\mathrm{H}}$). This, in conjunction with the relatively low magnitude of correlation energy predicted by ASCI relative to other methods, indicates that the extrapolated ASCI error bar estimate is much too small in this case. This is likely a consequence of the stubbornly large $E_{PT2}$ values for the variational subspace sizes considered (as can be seen from Table S7), which likely prevents attainment of the asymptotic $E_{PT2} \rightarrow 0$ regime behavior for the extrapolation (despite $r^2$ of the linear fit being very close to 1, which is the origin of the too small error bars). It is however also worth noting that the extrapolation protocol nonetheless is quite effective, recovering $\sim -25/-26$ m$E_{\mathrm{H}}$ of the $\sim -28$ m$E_{\mathrm{H}}$ correlation not recovered by ASCI+PT2 alone (assuming an actual correlation energy of $\sim -863$ m$E_{\mathrm{H}}$). More reliable estimates from ASCI+PT2 would require larger variational subspaces than those studied in this work. Our original choice was partly

determined by code limitations, though we considered $5 \times 10^6$ determinants to be sufficient at the time of the blind challenge.

**Table S7:** Correlation energies ($E_c$, in m$E_H$) for ASCI wave functions with various number of determinants ($N_{dets}$).

| Delocalized Orbitals (original blind test) | | | | Localized orbitals | | | |
|---|---|---|---|---|---|---|---|
| $N_{dets}$ | $E_c^{var}$ | $E_c^{PT2}$ | $E_c^{var+PT2}$ | $N_{dets}$ | $E_c^{var}$ | $E_c^{PT2}$ | $E_c^{var+PT2}$ |
| $1 \times 10^5$ | −661.17 | −159.97 | −821.14 | $1 \times 10^5$ | −698.31 | −116.74 | −815.05 |
| $2.5 \times 10^5$ | −685.91 | −139.54 | −825.45 | $2.5 \times 10^5$ | −719.63 | −101.03 | −820.65 |
| $5 \times 10^5$ | −698.34 | −129.41 | −827.75 | $5 \times 10^5$ | −735.12 | −89.49 | −824.62 |
| $1 \times 10^6$ | −709.96 | −120.04 | −830.00 | $1 \times 10^6$ | −749.43 | −79.17 | −828.60 |
| $2 \times 10^6$ | −721.68 | −110.61 | −832.29 | $2 \times 10^6$ | −761.51 | −70.49 | −832.00 |
| $5 \times 10^6$ | −737.13 | −98.25 | −835.38 | $4 \times 10^6$ | −772.35 | −62.83 | −835.18 |
| Fit | | | $-860.0 \pm 0.2$ | Fit | | | $-861.3 \pm 0.5$ |

# 9 iCI

The iCI approach,[S55,S56] which was born from the restricted static-dynamic-static[S57] (SDS) framework for treating strongly correlated electrons, is a method designed to converge from above to the FCI limit within just a few iterations, by constructing and diagonalizing a $3N_P \times 3N_P$ Hamiltonian matrix at each macro/micro-iteration, even when starting with a very poor initial guess. Here, $N_P$ denotes the number of target states. This convergence behaviour is hardly surprising, since the lowest order realization of the SDS framework, i.e., SDSPT2,[S58] already performs very well for prototypical systems of variable near degeneracies. However, iCI is computationally very expensive. One way out is to combine iCI with the idea of configuration selection, so as to generate a compact variational space for static correlation. The remaining dynamic correlation is treated via Epstein-Nesbet PT2. In brief, iCI has the following features: **(i)** Full spin symmetry is always maintained by taking configuration state functions (CSF) as the many-electron basis. **(ii)** Although the selection is performed on individual CSFs, it is orbital configurations (oCFG) that are used as the organizing units. **(iii)** Given a coefficient pruning threshold, $C_{min}$ (which determines the size

of the variational space for static correlation), the selection of important oCFGs/CSFs is performed iteratively until convergence. **(iv)** At each iteration in the growth of the wave function, the first-order interacting space is decomposed into disjoint subspaces, so as to reduce memory requirement on one hand and facilitate parallelization on the other. **(v)** Upper bounds (which involve only two-electron integrals) for the interactions between doubly connected oCFG pairs are used to screen each first-order interacting subspace before the first-order coefficients of individual CSFs are evaluated. **(vi)** The diagonalization of the Hamiltonian matrix in the variational space is achieved by the iterative vector interaction (iVI) method[S59,S60] (which, for $N_p$ roots, constructs and diagonalizes a $3N_p \times 3N_p$ matrix in each iteration). **(vii)** Upon termination of the selection, dynamic correlation is estimated by using state-specific Epstein-Nesbet PT2 (iCIPT2). Results were obtained in $D_{2\mathrm{h}}$ point group symmetry using either HF or natural (NO) orbitals, cf. Fig. S7, of which the linearly extrapolated (using the last six data points) iCIPT2(NO) result of $\Delta E_{\mathrm{iCIPT2(NO)}} = -861.05 \pm 0.5$ m$E_{\mathrm{H}}$ is used in Fig. 1 of the main text, cf. Table S8 and Fig. S8. Calculations were run using BDF (Beijing Density Functional) program[S61,S62] on a single node with two Intel Xeon E5-2640 v3 processors (16 cores @ 2.6 GHz, 8.0 GB/core), and the OpenMP efficiency was approximately 50 %.

Following the submission of the iCI result in Fig. 1 of the main text (Ref. S56), the efficiency of the method was increased by a factor of nearly 20. As such, the same $C_{\mathrm{min}}$ values now always lead to smaller variational space, which has allowed for larger calculations than what was previously possible using either canonical HF orbitals or NOs. These updated results (not part of the blind challenge) are also presented in Fig. S7 (with dashed lines), cf. also Table S10 and Fig. S9. These are estimated to be more accurate than the original results since the selected variational space is larger. Moreover, the updated iCIPT2(NO) results are again estimated to be more reliable than the corresponding iCIPT2(HF) results since the former are always lower than the latter for each considered $C_{\mathrm{min}}$ value. Furthermore, the gap

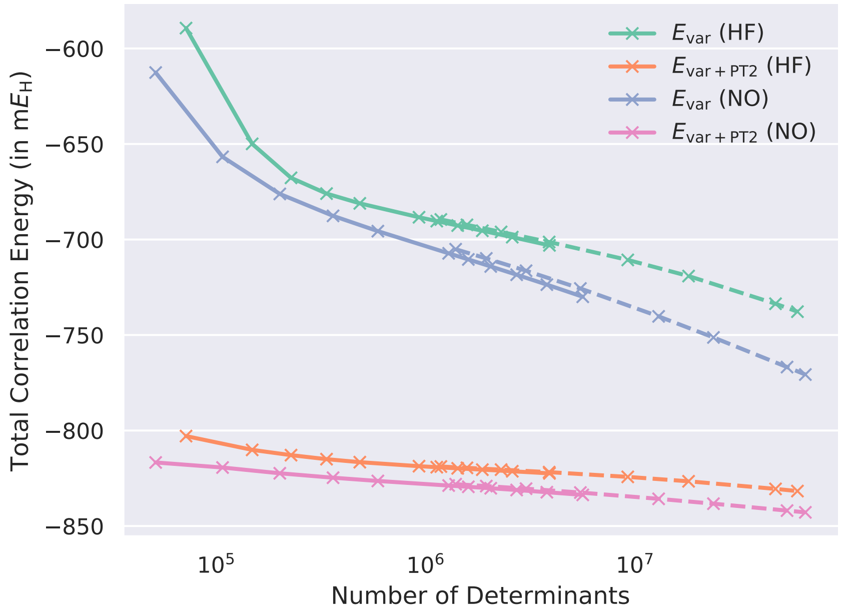


**Figure S7:** iCI results. Original results are plotted with solid lines, updated results (not part of main study) are plotted with dashed lines.

between the smallest $C_{\text{min}}$ value and the extrapolated value is smaller for iCIPT2(NO) than for iCIPT2(HF). The linear extrapolations (again not shown) yield final correlation energies of $\Delta E_{\text{iCIPT2(HF,new)}} = -866.07 \pm 1.0$ m$E_{\text{H}}$ and $\Delta E_{\text{iCIPT2(NO,new)}} = -864.15 \pm 0.6$ m$E_{\text{H}}$.

For both the original and the updated results, the remaining difference between HF- and NO-based iCIPT2 (ca. 2 m$E_{\text{H}}$) may be understood in terms of space dimensions, as the cumulative effect of the unsampled CSFs remains substantial. To verify this argument, $Cr_2$/Ahlrichs-SVP may be used as an example. The difference between iCIPT2(HF) and iCIPT2(NO) in this case is within 0.1 m$E_{\text{H}}$, correlating with the fact that the sampled space of CSFs makes up a considerably larger part of the FCI Hilbert space.

# 10 FCCR

The size-extensive FCCR method exploits screenings within the single-reference CC formalism for constructing the excitation manifold ($\mathcal{P}$) and to exclude insignificant operation

**Table S8:** iCIPT2 blind-test correlation energies for benzene with natural orbitals

| $C_{min}$ | $N_{cfg}$ | $\tilde{N}_{csf}$ [a] | $\tilde{N}_{det}$ [b] | $E_c^{var}/mE_H$ | $E_c^{PT2}/mE_H$ | $E_c/mE_H$ | $T/s$ [c] |
|---|---|---|---|---|---|---|---|
| $1.0 \times 10^{-3}$ | 14496 | 17890 | 50944 | −612.591 | −204.133 | −816.724 | 379 |
| $5.0 \times 10^{-4}$ | 28188 | 36448 | 106317 | −656.729 | −162.637 | −819.366 | 669 |
| $3.0 \times 10^{-4}$ | 48373 | 65080 | 199486 | −676.147 | −146.237 | −822.384 | 1481 |
| $2.0 \times 10^{-4}$ | 78947 | 109831 | 358274 | −687.627 | −137.072 | −824.699 | 2794 |
| $1.5 \times 10^{-4}$ | 119580 | 170356 | 586272 | −695.623 | −130.780 | −826.403 | 5066 |
| $1.0 \times 10^{-4}$ | 234640 | 344959 | 1277001 | −707.243 | −121.564 | −828.807 | 15206 |
| $9.0 \times 10^{-5}$ | 284068 | 421316 | 1585683 | −710.440 | −119.020 | −829.460 | 22335 |
| $8.0 \times 10^{-5}$ | 353743 | 529909 | 2028558 | −714.110 | −116.113 | −830.223 | 38399 |
| $7.0 \times 10^{-5}$ | 456337 | 692215 | 2697171 | −718.441 | −112.694 | −831.135 | 49238 |
| $6.0 \times 10^{-5}$ | 615593 | 947846 | 3759324 | −723.616 | −108.673 | −832.289 | 77344 |
| $5.0 \times 10^{-5}$ | 878837 | 1381837 | 5580152 | −729.983 | −103.707 | −833.690 | 133551 |
| 0.0[b] | | | | | | −861.05 ± 0.51 | |

[a] Number of selected CSFs.
[b] Estimated number of determinants according to the expression $\sum_I \frac{\tilde{N}^I_{csf}}{N^I_{csf}} N^I_{det}$, with $N^I_{det}$, $N^I_{csf}$ and $\tilde{N}^I_{csf}$ being the numbers of determinants, CSFs and selected CSFs of orbital configuration (oCFG) $I$, respectively.
[c] (1) CPU: Intel(R) Xeon(R) E5–2640 v3×2, 16 cores; (2) memory: 128 Gb; (3) parallelization: OpenMP, 16 threads.
[d] Linearly extrapolated result using values of the 9 smallest $C_{min}$. The error bar refers to the half length of 95% confidence interval.

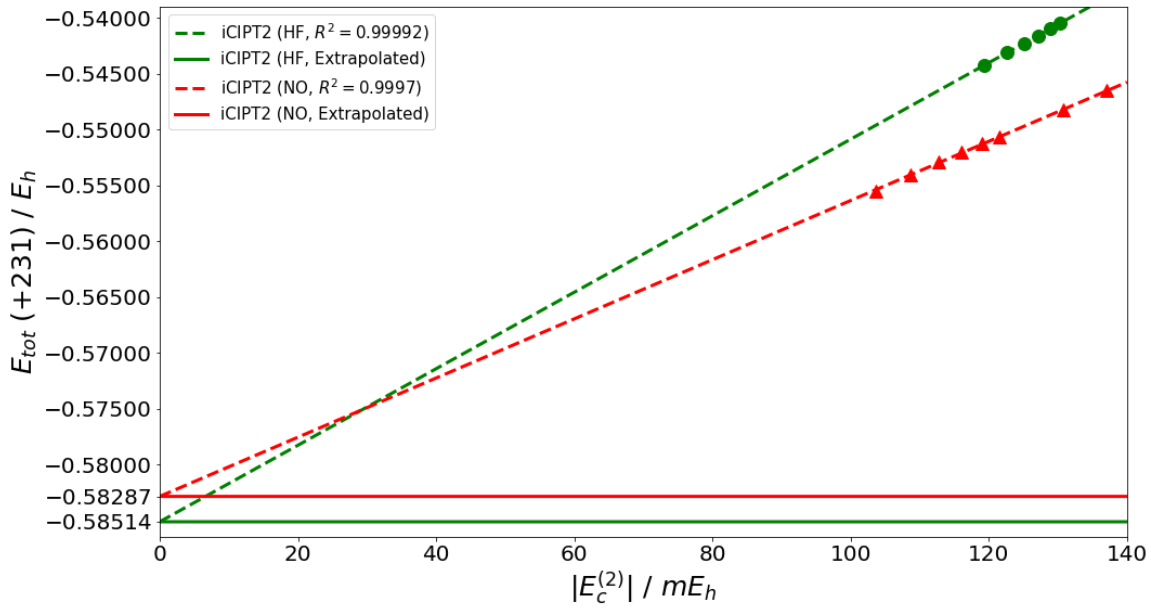


**Figure S8:** Linear fit of the correlation energy of benzene (blind test).

**Table S9:** iCIPT2 blind-test correlation energies for benzene with Hartree-Fock orbitals

| $C_{min}$ | $N_{cfg}$ | $\tilde{N}_{csf}$[a] | $\tilde{N}_{det}$[b] | $E_c^{var}/mE_H$ | $E_c^{PT2}/mE_H$ | $E_c/mE_H$ | $T/s$[c] |
|---|---|---|---|---|---|---|---|
| $1.0 \times 10^{-3}$ | 19811 | 24862 | 71137 | −589.336 | −213.573 | −802.909 | 301 |
| $5.0 \times 10^{-4}$ | 38400 | 51025 | 147228 | −649.922 | −160.205 | −810.127 | 837 |
| $3.0 \times 10^{-4}$ | 54907 | 76712 | 225685 | −667.714 | −145.170 | −812.884 | 1309 |
| $2.0 \times 10^{-4}$ | 75868 | 109263 | 333495 | −675.959 | −139.038 | −814.997 | 2363 |
| $1.5 \times 10^{-4}$ | 103807 | 150972 | 480806 | −681.083 | −135.481 | −816.564 | 3036 |
| $1.0 \times 10^{-4}$ | 180981 | 269149 | 921928 | −688.358 | −130.306 | −818.664 | 9875 |
| $9.0 \times 10^{-5}$ | 214438 | 320658 | 1120558 | −690.363 | −128.831 | −819.194 | 12712 |
| $8.0 \times 10^{-5}$ | 261828 | 394778 | 1410356 | −692.695 | −127.102 | −819.797 | 17447 |
| $7.0 \times 10^{-5}$ | 331831 | 505250 | 1849734 | −695.422 | −125.065 | −820.487 | 26334 |
| $6.0 \times 10^{-5}$ | 444010 | 683971 | 2570589 | −698.767 | −122.563 | −821.330 | 42053 |
| $5.0 \times 10^{-5}$ | 640800 | 1001148 | 3869123 | −703.066 | −119.361 | −822.427 | 72945 |
| 0.0[b] | | | | | | $-863.32 \pm 0.54$ | |

[a] Number of selected CSFs.

[b] Estimated number of determinants according to the expression $\sum_I \frac{\tilde{N}_{csf}^I}{N_{csf}^I} N_{det}^I$, with $N_{det}^I$, $N_{csf}^I$ and $\tilde{N}_{csf}^I$ being the numbers of determinants, CSFs and selected CSFs of orbital configuration (oCFG) $I$, respectively.

[c] (1) CPU: Intel(R) Xeon(R) E5–2640 v3×2, 16 cores; (2) memory: 128 Gb; (3) parallelization: OpenMP, 16 threads.

[d] Linearly extrapolated result using values of the 6 smallest $C_{min}$. The error bar refers to the half length of 95% confidence interval.

**Table S10:** iCIPT2 correlation energies for benzene with natural orbitals (updated results).

| $C_{min}$ | $N_{cfg}$ | $\tilde{N}_{csf}$[a] | $\tilde{N}_{det}$[b] | $E_c^{var}/mE_H$ | $E_c^{PT2}/mE_H$ | $E_c/mE_H$ | $T/s$[c] |
|---|---|---|---|---|---|---|---|
| $6.0 \times 10^{-5}$ | 245224 | 379662 | 1379097 | −705.099 | −122.996 | −828.095 | 491 |
| $5.0 \times 10^{-5}$ | 330089 | 518448 | 1932040 | −709.899 | −119.182 | −829.081 | 670 |
| $4.0 \times 10^{-5}$ | 486177 | 778940 | 2991370 | −716.354 | −114.087 | −830.441 | 1039 |
| $3.0 \times 10^{-5}$ | 830917 | 1369463 | 5436028 | −725.650 | −106.817 | −832.467 | 1834 |
| $2.0 \times 10^{-5}$ | 1809463 | 3121693 | 12849733 | −740.245 | −95.513 | −835.758 | 4273 |
| $1.5 \times 10^{-5}$ | 3134922 | 5595481 | 23479710 | −751.271 | −87.026 | −838.298 | 7597 |
| $1.0 \times 10^{-5}$ | 6555147 | 12315752 | 52744912 | −766.783 | −75.134 | −841.918 | 19299 |
| $9.0 \times 10^{-6}$ | 7869797 | 14995161 | 64497488 | −770.695 | −72.139 | −842.834 | 33344 |
| 0.0[d] | | | | | | $-864.15 \pm 0.57$ | |

[a] Number of selected CSFs.

[b] Estimated number of determinants according to the expression $\sum_I \frac{\tilde{N}_{csf}^I}{N_{csf}^I} N_{det}^I$, with $N_{det}^I$, $N_{csf}^I$ and $\tilde{N}_{csf}^I$ being the numbers of determinants, CSFs and selected CSFs of orbital configuration (oCFG) $I$, respectively.

[c] (1) CPU: Intel(R) Xeon(R) Gold 6240 ×4, 72 cores; (2) memory: 768 Gb; (3) parallelization: OpenMP, 72 threads.

[d] Linearly extrapolated result using values of the 6 smallest $C_{min}$. The error bar refers to the half length of 95% confidence interval.

**Table S11:** iCIPT2 correlation energies for benzene with Hartree-Fock orbitals (updated results).

| $C_{\rm min}$ | $N_{\rm cfg}$ | $\tilde{N}_{\rm csf}$ [a] | $\tilde{N}_{\rm det}$ [b] | $E_{\rm c}^{\rm var}/{\rm m}E_{\rm H}$ | $E_{\rm c}^{\rm PT2}/{\rm m}E_{\rm H}$ | $E_{\rm c}/{\rm m}E_{\rm H}$ | $T/s$ [c] |
|---|---|---|---|---|---|---|---|
| $6.0 \times 10^{-5}$ | 221314 | 338334 | 1172202 | −689.523 | −129.322 | −818.846 | 326 |
| $5.0 \times 10^{-5}$ | 282405 | 439038 | 1561473 | −692.337 | −127.201 | −819.539 | 426 |
| $4.0 \times 10^{-5}$ | 391414 | 620645 | 2273564 | −696.048 | −124.424 | −820.473 | 621 |
| $3.0 \times 10^{-5}$ | 631646 | 1017094 | 3856238 | −701.315 | −120.475 | −821.790 | 1109 |
| $2.0 \times 10^{-5}$ | 1398298 | 2301712 | 9150757 | −710.687 | −113.578 | −824.265 | 2749 |
| $1.5 \times 10^{-5}$ | 2583842 | 4359388 | 17861976 | −719.137 | −107.437 | −826.574 | 5387 |
| $1.0 \times 10^{-5}$ | 6206395 | 10978445 | 46457235 | −733.630 | −96.926 | −830.557 | 14470 |
| $9.0 \times 10^{-6}$ | 7736950 | 13878500 | 59119837 | −737.772 | −93.920 | −831.692 | 20203 |
| 0.0[b] | | | | | | −866.07 ± 0.99 | |

[a] Number of selected CSFs.

[b] Estimated number of determinants according to the expression $\sum_I \frac{\tilde{N}^I_{\rm csf}}{N^I_{\rm csf}} N^I_{\rm det}$, with $N^I_{\rm det}$, $N^I_{\rm csf}$ and $\tilde{N}^I_{\rm csf}$ being the numbers of determinants, CSFs and selected CSFs of orbital configuration (oCFG) $I$, respectively.

[c] (1) CPU: Intel(R) Xeon(R) Gold 6240 ×4, 72 cores; (2) memory: 768 Gb; (3) parallelization: OpenMP, 72 threads.

[d] Linearly extrapolated result using values of the 6 smallest $C_{min}$. The error bar refers to the half length of 95% confidence interval.

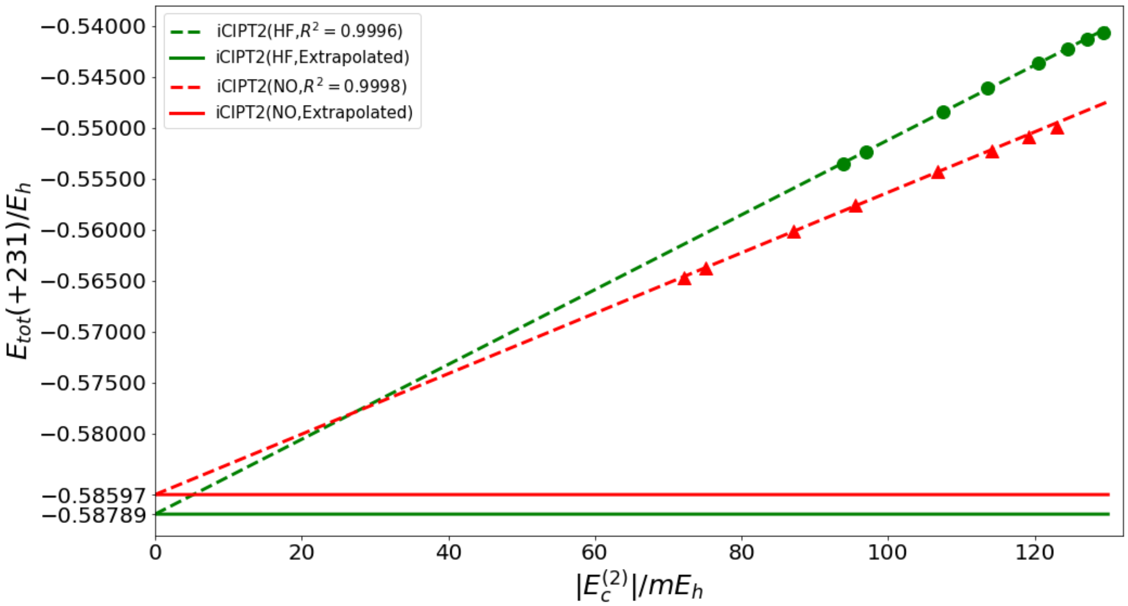


**Figure S9:** Linear fit of the correlation energy of benzene (updated results).

**Table S12:** Linearly extrapolated iCIPT2 correlation energies ($E_c$ in m$E_H$) for benzene and extrapolation errors (in m$E_H$). A: extrapolation distance; B: standard deviation; C: half length of 95% confidence interval.

| | Orbitals | $E_c$ | A | B | C | CPU/h | memory/Gb |
|---|---|---|---|---|---|---|---|
| Blind Test | NO | −861.05 | 27.36 | 0.22 | 0.51 | 1545 | ∼650 |
| | HF | −863.32 | 40.89 | 0.19 | 0.54 | 836 | ∼650 |
| Updated | NO | −864.15 | 21.32 | 0.21 | 0.57 | 1348 | ∼610 |
| | HF | −866.07 | 34.38 | 0.36 | 0.99 | 891 | ∼610 |

mostly arising from the nonlinear terms of the working equation.[S63] The subsequent FCCR(2) computes the second-order perturbative correction to FCCR using the entire interacting space ($\mathcal{Q}$) orthogonal to $\mathcal{P}$ generated through $[\hat{H}, \hat{T}_{\text{FCCR}}]$.[S64] For single-reference systems, FCCR(2') which approximate the $\hat{\lambda}$ amplitudes by $\hat{T}^{\dagger}$ is also available. All calculations were performed using the `GELLAN` program[S65] in parallel on Intel Xeon Gold 6148 nodes (40 cores @ 2.4 GHz).

**Table S13:** FCCR calculation details (blind test).

| Method | $\Delta E$/m$E_H$ |
|---|---|
| FCCR(MP) | −860.1 |
| FCCR(EN) | −865.4 |
| FCCR(avg) | −862.8 |
| FCCR(avg) + $\vartheta_{\mathcal{O}}$ corr. | −863.0 |

Table S13 shows the result of FCCR(2') with the Møller-Plesset (MP) and Epstein-Nesbet (EN) partitionings with the connectivity threshold $\vartheta_{\mathcal{C}} = 0.03$ and the operation threshold $\vartheta_{\mathcal{O}} = 3.0 \times 10^{-7}$ as combined with the exclusion-principle-violating (EPV) form of the screening,[S63] leading to 4,818,644 FCCR cluster amplitudes. The FCI energy is estimated to lie very close to the average of the MP and EN results from various benchmarks (avg.), which may further be corrected for $\vartheta_{\mathcal{O}}$ based on CCSD, resulting in the estimate $-862.98$m$E_H$. This calculation required 0.1M core hours invoking 640 MPI processes. The interacting space $\mathcal{Q}$ for the second-order correction is perfectly distributed to the processes,

and the memory requirement of the present FCCR(2') calculation is at most 2GB per process.

**Table S14:** FCCR calculation details (updated results).

| $\vartheta_{\mathcal{P}}$ | $\Delta E/\mathrm{m}E_{\mathrm{H}}$ | $N_{\mathcal{P}}$ | $E^{(2)}/\mathrm{m}E_{\mathrm{H}}$ | $N_{\mathcal{Q}}$ |
|---|---|---|---|---|
| $5 \times 10^{-4}$ | −849.05 | 109,860 | −81.09 | $2.2 \times 10^{8}$ |
| $4 \times 10^{-4}$ | −852.25 | 137,421 | −62.36 | $2.6 \times 10^{8}$ |
| $3 \times 10^{-4}$ | −854.93 | 174,914 | −46.71 | $3.7 \times 10^{8}$ |
| $2 \times 10^{-4}$ | −856.84 | 229,842 | −35.11 | $6.4 \times 10^{8}$ |
| extrap. | −862.83 | — | 0.0 | — |

A fast and more systematic estimate of the FCI limit is enabled by the extrapolation of FCCR(2). Table S14 presents an updated FCCR(2) correlation energy (not part of the blind challenge) along with the second-order correction of the MP partitioning as a function of the principal screening threshold $\vartheta_{\mathcal{P}}$. Besides $\vartheta_{\mathcal{O}}$, the latest implementation of FCCR(2) controls the excitation manifold in terms of the two screening parameters, $\vartheta_{\mathcal{P}}$ to select the cluster operators of $\mathcal{P}$ perturbatively and $\vartheta_{\mathcal{G}}$ for the generator space ($\mathcal{G}$) to discriminate strong correlation in $\mathcal{P}$.[S64] Except for $\vartheta_{\mathcal{P}}$, all screening parameters are fixed to be $\vartheta_{\mathcal{G}} = 0.01$, $\vartheta_{\mathcal{O}} = 10^{-7}$ for FCCR, and $\vartheta_{\mathcal{O}} = 3.0 \times 10^{-6}$ for $E^{(2)}$. Tightening $\vartheta_{\mathcal{P}}$ increases the accuracy of FCCR(2) according to the increasing dimensions of $\mathcal{P}$ and $\mathcal{Q}$. It is found that a linear relationship holds[S64] between $\Delta E_{\mathrm{FCCR(2)}}$ and $E^{(2)}$, as shown in Fig. S10, and the best estimate of FCCR(2) based on the extrapolation is $-862.83$ m$E_{\mathrm{H}}$. The calculations for the four values of $\vartheta_{\mathcal{P}}$ in Table S14 required 0.035M, 0.048M, 0.073M and 0.134M core hours, respectively, using 640 MPI processes. The algorithmic details of the FCCR(2) implementation and other applications will be elaborated in a separate paper.[S64]

# 11 CCSDTQ

The CCSDTQ[S41,S42] correlation energy of $\Delta E_{\mathrm{CCSDTQ}} = -862.37$ m$E_{\mathrm{H}}$ was obtained using the `NCC` module of the `CFOUR` program[S66–S69] on a single Intel Xeon CPU E5-4620 node (8

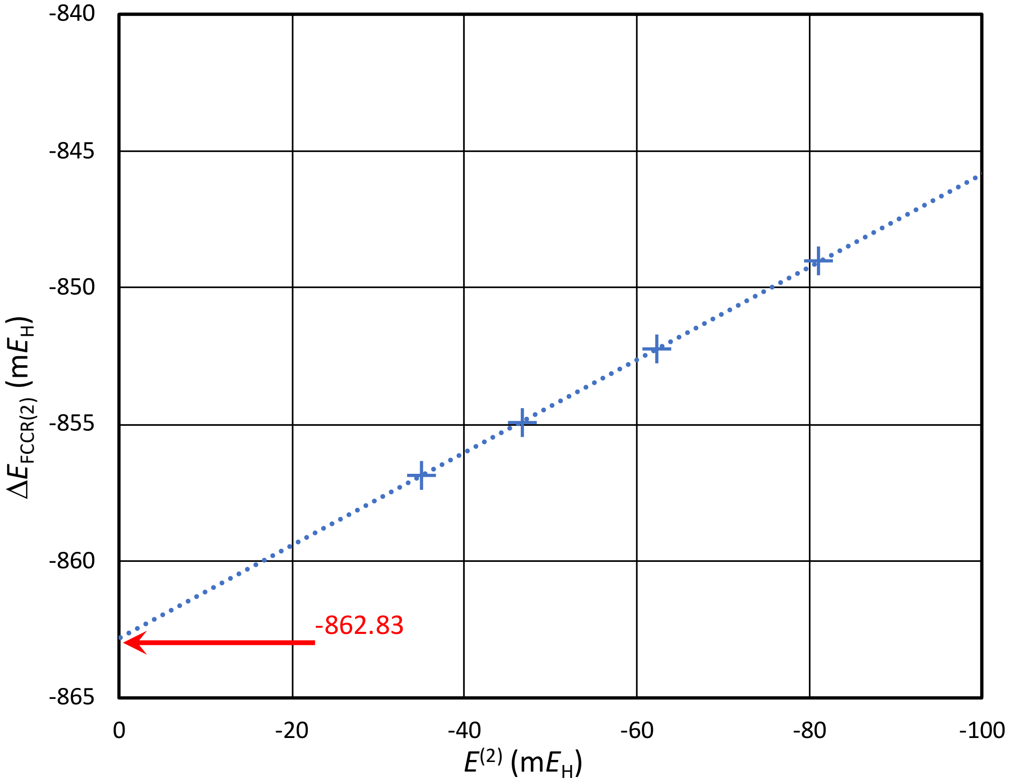


**Figure S10:** Updated FCCR results. The linear extrapolation of the FCCR(2) energy.

cores @ 2.2 GHz, 15.0 GB/core). Convergence was reached in 10 iterations.

# 12 Cluster Decomposition

**Table S15:** Cluster decomposition ($L_2$-norm) of a 5M-determinant ASCI wave function (with delocalized orbitals) for excitation levels $1 \leq n \leq 6$.

| $n$ | $\|\boldsymbol{c}_n\|$ | $\|\boldsymbol{t}_n\|$ | Ratio/% |
|---|---|---|---|
| 1 | 0.019477 | 0.019477 | 100.0 |
| 2 | 0.533103 | 0.533108 | 100.0 |
| 3 | 0.064742 | 0.065137 | 100.6 |
| 4 | 0.142888 | 0.014178 | 9.92 |
| 5 | 0.006201 | 0.000465 | 7.50 |
| 6 | 0.008792 | 0.001948 | 22.16 |

Table S15 presents results for a cluster decomposition[S70] of an ASCI wave function with

$5.0 \times 10^6$ determinants (using delocalized orbitals, as described in Sec 8). These results indicate that most of the $\{\boldsymbol{c}_4\}$ (and higher order) CI coefficients come from disconnected terms.

Subsequent to the main study, a cluster decomposition was also carried out on a $4.0 \times 10^6$ determinant ASCI wave function with localized orbitals (as described in Sec 8.1), as this CI wave function had a lower variational energy than the previous one ($-772$ m$E_\mathrm{H}$ correlation vs $-737$ m$E_\mathrm{H}$) and was thus a better approximation to the true FCI wave function. The resulting values are provided in Table S16, which differ slightly from those in Table S15. The general picture, however, remains the same, in that $\{\boldsymbol{c}_4\}$ and higher order excitations seem to mostly arise from disconnected terms.

**Table S16:** Cluster decomposition ($L_2$-norm) of a 4M-determinant ASCI wave function (with localized orbitals) for excitation levels $1 \leq n \leq 6$.

| $n$ | $\lvert\boldsymbol{c}_n\rvert$ | $\lvert\boldsymbol{t}_n\rvert$ | Ratio/% |
|---|---|---|---|
| 1 | 0.01777 | 0.01777 | 100.0 |
| 2 | 0.55063 | 0.55063 | 100.0 |
| 3 | 0.06855 | 0.06868 | 100.2 |
| 4 | 0.16486 | 0.01755 | 10.65 |
| 5 | 0.00903 | 0.00076 | 8.38 |
| 6 | 0.01610 | 0.00259 | 16.11 |

# References


(S1) Schreiber, M.; Silva-Junior, M. R.; Sauer, S. P. A.; Thiel, W. Benchmarks for Electronically Excited States: CASPT2, CC2, CCSD, and CC3. J. Chem. Phys. **2008**, 128, 134110.

(S2) Eriksen, J. J.; Lipparini, F.; Gauss, J. Virtual Orbital Many-Body Expansions: A Possible Route towards the Full Configuration Interaction Limit. J. Phys. Chem. Lett. **2017**, 8, 4633.

(S3) Eriksen, J. J.; Gauss, J. Many-Body Expanded Full Configuration Interaction. I. Weakly Correlated Regime. J. Chem. Theory Comput. **2018**, 14, 5180.

(S4) Eriksen, J. J.; Gauss, J. Many-Body Expanded Full Configuration Interaction. II. Strongly Correlated Regime. J. Chem. Theory Comput. **2019**, 15, 4873.

(S5) Eriksen, J. J.; Gauss, J. Generalized Many-Body Expanded Full Configuration Interaction Theory. J. Phys. Chem. Lett. **2019**, 10, 7910.

(S6) `PyMBE`: A Many-Body Expanded Correlation Code by Janus Juul Eriksen, See `https://gitlab.com/januseriksen/pymbe`.

(S7) Pipek, J.; Mezey, P. G. A Fast Intrinsic Localization Procedure Applicable for *Ab Initio* and Semiempirical Linear Combination of Atomic Orbital Wave Functions. J. Chem. Phys. **1989**, 90, 4916.

(S8) Chan, G. K.-L.; Sharma, S. The Density Matrix Renormalization Group in Quantum Chemistry. Ann. Rev. Phys. Chem. **2011**, 62, 465.

(S9) Wouters, S.; Van Neck, D. The Density Matrix Renormalization Group for *Ab Initio* Quantum Chemistry. Eur. Phys. J. D **2014**, 68, 272.

(S10) Knecht, S.; Hedegård, E. D.; Keller, S.; Kovyrshin, A.; Ma, Y.; Muolo, A.; Stein, C. J.; Reiher, M. New Approaches for *Ab Initio* Calculations of Molecules with Strong Electron Correlation. Chimia **2016**, 70, 244.

(S11) Chan, G. K.-L.; Head-Gordon, M. Highly Correlated Calculations with a Polynomial Cost Algorithm: A Study of the Density Matrix Renormalization Group. J. Chem. Phys. **2002**, 116, 4462.

(S12) Chan, G. K.-L. An Algorithm for Large Scale Density Matrix Renormalization Group Calculations. J. Chem. Phys. **2004**, 120, 3172.

(S13) Ghosh, D.; Hachmann, J.; Yanai, T.; Chan, G. K.-L. Orbital Optimization in the Density Matrix Renormalization Group, with Applications to Polyenes and $\beta$-Carotene. J. Chem. Phys. **2008**, 128, 144117.

(S14) Sharma, S.; Chan, G. K.-L. Spin-Adapted Density Matrix Renormalization Group Algorithms for Quantum Chemistry. J. Chem. Phys. **2012**, 136, 124121.

(S15) Olivares-Amaya, R.; Hu, W.; Nakatani, N.; Sharma, S.; Yang, J.; Chan, G. K.-L. The *Ab-Initio* Density Matrix Renormalization Group in Practice. J. Chem. Phys. **2015**, 142, 034102.

(S16) `PySCF`: The Python-Based Simulations of Chemistry Framework, See `https://pyscf.github.io/`.

(S17) Sun, Q.; Berkelbach, T. C.; Blunt, N. S.; Booth, G. H.; Guo, S.; Li, Z.; Liu, J.; McClain, J.; Sayfutyarova, E. R.; Sharma, S.; Wouters, S.; Chan, G. K.-L. PySCF: The Python-Based Simulations of Chemistry Framework. WIREs Comput. Mol. Sci. **2018**, 8, e1340.

(S18) Sun, Q.; Zhang, X.; Banerjee, S.; Bao, P.; Barbry, M.; Blunt, N. S.; Bogdanov, N. A.; Booth, G. H.; Chen, J.; Cui, Z.-H.; Eriksen, J. J.; Gao, Y.; Guo, S.; Hermann, J.;

Hermes, M. R.; Koh, K.; Koval, P.; Lehtola, S.; Li, Z.; Liu, J.; Mardirossian, N.; McClain, J. D.; Motta, M.; Mussard, B.; Pham, H. Q.; Pulkin, A.; Purwanto, W.; Robinson, P. J.; Ronca, E.; Sayfutyarova, E.; Scheurer, M.; Schurkus, H. F.; Smith, J. E. T.; Sun, C.; Sun, S.-N.; Upadhyay, S.; Wagner, L. K.; Wang, X.; White, A.; Whitfield, J. D.; Williamson, M. J.; Wouters, S.; Yang, J.; Yu, J. M.; Zhu, T.; Berkelbach, T. C.; Sharma, S.; Sokolov, A.; Chan, G. K.-L. Recent Developments in the PySCF Program Package. J. Chem. Phys. **2020**, 153, 024109.

(S19) Edmiston, C.; Ruedenberg, K. Localized Atomic and Molecular Orbitals. Rev. Mod. Phys. **1963**, 35, 457.

(S20) Ghanem, K.; Lozovoi, A. Y.; Alavi, A. Unbiasing the Initiator Approximation in Full Configuration Interaction Quantum Monte Carlo. J. Chem. Phys. **2019**, 151, 224108.

(S21) H. Booth, A. Alavi *et al.*, Standalone `NECI` Codebase Designed for FCIQMC and other Stochastic Quantum Chemistry Methods, 2013, See `https://github.com/ghb24/NECI_STABLE`.

(S22) Guther, K.; Anderson, R. J.; Blunt, N. S.; Bogdanov, N. A.; Cleland, D.; Dattani, N.; Dobrautz, W.; Ghanem, K.; Jeszenszki, P.; Liebermann, N.; Manni, G. L.; Lozovoi, A. Y.; Luo, H.; Ma, D.; Merz, F.; Overy, C.; Rampp, M.; Samanta, P. K.; Schwarz, L. R.; Shepherd, J. J.; Smart, S. D.; Vitale, E.; Weser, O.; Booth, G. H.; Alavi, A. `NECI`: $N$-Electron Configuration Interaction with an Emphasis on State-of-the-Art Stochastic Methods. J. Chem. Phys. **2020**, 153, 034107.

(S23) Deustua, J. E.; Magoulas, I.; Shen, J.; Piecuch, P. Communication: Approaching Exact Quantum Chemistry by Cluster Analysis of Full Configuration Interaction Quantum Monte Carlo Wave Functions. J. Chem. Phys. **2018**, 149, 151101.

(S24) Booth, G. H.; Thom, A. J. W.; Alavi, A. Fermion Monte Carlo without Fixed Nodes:

A Game of Life, Death, and Annihilation in Slater Determinant Space. J. Chem. Phys. **2009**, 131, 054106.

(S25) Cleland, D.; Booth, G. H.; Alavi, A. Communications: Survival of the Fittest: Accelerating Convergence in Full Configuration-Interaction Quantum Monte Carlo. J. Chem. Phys. **2010**, 132, 041103.

(S26) Thom, A. J. W. Stochastic Coupled Cluster Theory. Phys. Rev. Lett. **2010**, 105, 263004.

(S27) Franklin, R. S. T.; Spencer, J. S.; Zoccante, A.; Thom, A. J. W. Linked Coupled Cluster Monte Carlo. J. Chem. Phys. **2016**, 144, 044111.

(S28) Deustua, J. E.; Shen, J.; Piecuch, P. Converging High-Level Coupled-Cluster Energetics by Monte Carlo Sampling and Moment Expansions. Phys. Rev. Lett. **2017**, 119, 223003.

(S29) Deustua, J. E.; Yuwono, S. H.; Shen, J.; Piecuch, P. Accurate Excited-State Energetics by a Combination of Monte Carlo Sampling and Equation-of-Motion Coupled-Cluster Computations. J. Chem. Phys. **2019**, 150, 111101.

(S30) Yuwono, S. H.; Chakraborty, A.; Deustua, J. E.; Shen, J.; Piecuch, P. Accelerating Convergence of Equation-of-Motion Coupled-Cluster Computations Using the Semi-Stochastic CC($P$;$Q$) Formalism. Mol. Phys., **2020**, e1817592, published online: 17 Sep 2020, DOI: 10.1080/00268976.2020.1817592.

(S31) Paldus, J.; Čížek, J.; Takahashi, M. Approximate Account of the Connected Quadruply Excited Clusters in the Coupled-Pair Many-Electron Theory. Phys. Rev. A **1984**, 30, 2193–2209.

(S32) Piecuch, P.; Paldus, J. Coupled Cluster Approaches with an Approximate Account

of Triexcitations and the Optimized Inner Projection Technique. Theor. Chim. Acta **1990**, 78, 65–128.

(S33) Piecuch, P.; Toboła, R.; Paldus, J. Approximate Account of Connected Quadruply Excited Clusters in Single-Reference Coupled-Cluster Theory via Cluster Analysis of the Projected Unrestricted Hartree-Fock Wave Function. Phys. Rev. A **1996**, 54, 1210–1241.

(S34) Paldus, J.; Planelles, J. Valence Bond Corrected Single Reference Coupled Cluster Approach. I. General Formalism. Theor. Chim. Acta **1994**, 89, 13–31.

(S35) Stolarczyk, L. Z. Complete Active Space Coupled-Cluster Method. Extension of Single-Reference Coupled-Cluster Method Using the CASSCF Wavefunction. Chem. Phys. Lett. **1994**, 217, 1–6.

(S36) Peris, G.; Planelles, J.; Paldus, J. Single-Reference CCSD Approach Employing Three- and Four-Body CAS SCF Corrections: A Preliminary Study of a Simple Model. Int. J. Quantum Chem. **1997**, 62, 137–151.

(S37) Peris, G.; Planelles, J.; Malrieu, J.-P.; Paldus, J. Perturbatively Selected CI as an Optimal Source for Externally Corrected CCSD. J. Chem. Phys. **1999**, 110, 11708–11716.

(S38) Li, X.; Paldus, J. Reduced Multireference CCSD Method: An Effective Approach to Quasidegenerate States. J. Chem. Phys. **1997**, 107, 6257–6269.

(S39) Li, X.; Paldus, J. Reduced Multireference Coupled Cluster Method with Singles and Doubles: Perturbative Corrections for Triples. J. Chem. Phys. **2006**, 124, 174101.

(S40) Purvis, III, G. D.; Bartlett, R. J. A Full Coupled-Cluster Singles and Doubles Model: The Inclusion of Disconnected Triples. J. Chem. Phys. **1982**, 76, 1910–1918.

(S41) Oliphant, N.; Adamowicz, L. Coupled-Cluster Method Truncated at Quadruples. J. Chem. Phys. **1991**, 95, 6645–6651.

(S42) Kucharski, S. A.; Bartlett, R. J. The Coupled-Cluster Single, Double, Triple, and Quadruple Excitation Method. J. Chem. Phys. **1992**, 97, 4282–4288.

(S43) Piecuch, P.; Paldus, J. On the Solution of Coupled-Cluster Equations in the Fully Correlated Limit of Cyclic Polyene Model. Int. J. Quantum Chem. **1991**, 40, 9–34.

(S44) Kats, D.; Manby, F. R. Communication: The Distinguishable Cluster Approximation. J. Chem. Phys. **2013**, 139, 021102.

(S45) Magoulas, I.; Deustua, J. E.; Shen, J.; Piecuch, P. Converging Exact Energetics in Strongly Correlated Systems by Cluster Analysis of Full Configuration Interaction Quantum Monte Carlo Wave Functions. In preparation.

(S46) Li, J.; Yao, Y.; Holmes, A.; Otten, M.; Sharma, S.; Umrigar, C. J. Accurate Many-Body Electronic Structure Near the Basis Set Limit: Application to the Chromium Dimer. Phys. Rev. Res. **2020**, 2, 012015(R).

(S47) Yao, Y.; Giner, E.; Li, J.; Toulouse, J.; Umrigar, C. J. Almost Exact Energies for the Gaussian-2 Set with the Semistochastic Heat-Bath Configuration Interaction Method. arXiv:arXiv:2004.10059 **2020**.

(S48) `Arrow`, a Semistochastic Heat-Bath Configuration Interaction (SHCI) Program, See `https://github.com/QMC-Cornell/shci`.

(S49) Tubman, N. M.; Freeman, C. D.; Levine, D. S.; Hait, D.; Head-Gordon, M.; Whaley, K. B. Modern Approaches to Exact Diagonalization and Selected Configuration Interaction with the Adaptive Sampling CI Method. J. Chem. Theory Comput. **2020**, 16, 2139.

(S50) Tubman, N. M.; Levine, D. S.; Hait, D.; Head-Gordon, M.; Whaley, K. B. An Efficient Deterministic Perturbation Theory for Selected Configuration Interaction Methods. arXiv:1808.02049 **2018**.

(S51) Shao, Y.; Gan, Z.; Epifanovsky, E.; Gilbert, A. T. B.; Wormit, M.; Kussmann, J.; Lange, A. W.; Behn, A.; Deng, J.; Feng, X., et al. Advances in Molecular Quantum Chemistry Contained in the Q-Chem 4 Program Package. Mol. Phys. **2015**, 113, 184.

(S52) Levine, D. S.; Hait, D.; Tubman, N. M.; Lehtola, S.; Whaley, K. B.; Head-Gordon, M. CASSCF with Extremely Large Active Spaces using the Adaptive Sampling Configuration Interaction Method. J. Chem. Theory Comput. **2020**, 16, 2340.

(S53) Hait, D.; Tubman, N. M.; Levine, D. S.; Whaley, K. B.; Head-Gordon, M. What Levels of Coupled Cluster Theory Are Appropriate for Transition Metal Systems? A Study Using Near-Exact Quantum Chemical Values for 3d Transition Metal Binary Compounds. J. Chem. Theory Comput. **2019**, 15, 5370.

(S54) Sano, T. Elementary Jacobi Rotation Method for Generalized Valence Bond Perfect-Pairing Calculations Combined with Simple Procedure for Generating Reliable Initial Orbitals. J. Mol. Struct.: THEOCHEM **2000**, 528, 177.

(S55) Liu, W.; Hoffmann, M. R. iCI: Iterative CI toward full CI. J. Chem. Theory Comput. **2016**, 12, 1169.

(S56) Zhang, N.; Liu, W.; Hoffmann, M. R. Iterative Configuration Interaction with Selection. J. Chem. Theory Comput. **2020**, 16, 2296.

(S57) Liu, W.; Hoffmann, M. R. SDS: The 'Static-Dynamic-Static' Framework for Strongly Correlated Electrons. Theor. Chem. Acc. **2014**, 133, 1481.

(S58) Lei, Y.; Liu, W.; Hoffmann, M. R. Further Development of SDSPT2 for Strongly Correlated Electrons. Mol. Phys. **2017**, 115, 2696.

(S59) Huang, C.; Liu, W.; Xiao, Y.; Hoffmann, M. R. iVI: An Iterative Vector Interaction Method for Large Eigenvalue Problems. J. Comput. Chem. **2017**, 38, 2481.

(S60) Huang, C.; Liu, W. iVI-TD-DFT: An Iterative Vector Interaction Method for Exterior/Interior Roots of TD-DFT. J. Comput. Chem. **2019**, 40, 1023.

(S61) Liu, W.; Hong, G.; Dai, D.; Li, L.; Dolg, M. The Beijing Four-Component Density Functional Program Package (BDF) and its Application to EuO, EuS, YbO and YbS. Theor. Chem. Acc. **1997**, 96, 75.

(S62) Zhang, Y.; Suo, B.; Wang, Z.; Zhang, N.; Li, Z.; Lei, Y.; Zou, W.; Gao, J.; Peng, D.; Pu, Z.; Xiao, Y.; Sun, Q.; Wang, F.; Ma, Y.; Wang, X.; Guo, Y.; Liu, W. BDF: A Relativistic Electronic Structure Program Package. J. Chem. Phys. **2020**, 152, 064113.

(S63) Xu, E.; Uejima, M.; Ten-no, S. L. Full Coupled-Cluster Reduction for Accurate Description of Strong Electron Correlation. Phys. Rev. Lett. **2018**, 121, 113001.

(S64) Xu, E.; Ten-no, S. L. *In Preparation* (2020).

(S65) `GELLAN`, a Hierarchical Massively-Parallel Quantum Chemistry Program, Kobe University.

(S66) Matthews, D. A.; Stanton, J. F. Accelerating the Convergence of Higher-Order Coupled Cluster Methods. J. Chem. Phys. **2015**, 143, 204103.

(S67) Matthews, D. A.; Stanton, J. F. Non-Orthogonal Spin-Adaptation of Coupled Cluster Methods: A New Implementation of Methods Including Quadruple Excitations. J. Chem. Phys. **2015**, 064108.

(S68) Matthews, D. A.; Cheng, L.; Harding, M. E.; Lipparini, F.; Stopkowicz, S.; Jagau, T.-C.; Szalay, P. G.; Gauss, J.; Stanton, J. F. Coupled-Cluster Techniques for Computational Chemistry: The CFOUR Program Package. J. Chem. Phys. **2020**, 152, 214108.

(S69) CFOUR, Coupled-Cluster Techniques for Computational Chemistry, a Quantum-Chemical Program Package by J. F. Stanton, J. Gauss, L. Cheng, M. E. Harding, D. A. Matthews, P. G. Szalay with Contributions from A. A. Auer, R. J. Bartlett, U. Benedikt, C. Berger, D. E. Bernholdt, Y. J. Bomble, O. Christiansen, F. Engel, R. Faber, M. Heckert, O. Heun, M. Hilgenberg, C. Huber, T.-C. Jagau, D. Jonsson, J. Jusélius, T. Kirsch, K. Klein, W. J. Lauderdale, F. Lipparini, T. Metzroth, L. A. Mück, D. P. O'Neill, D. R. Price, E. Prochnow, C. Puzzarini, K. Ruud, F. Schiffmann, W. Schwalbach, C. Simmons, S. Stopkowicz, A. Tajti, J. Vázquez, F. Wang, J. D. Watts and the integral packages MOLECULE (J. Almlöf and P. R. Taylor), PROPS (P. R. Taylor), ABACUS (T. Helgaker, H. J. Aa. Jensen, P. Jørgensen, and J. Olsen), and ECP routines by A. V. Mitin and C. van Wüllen. For the Current Version, see http://www.cfour.de.

(S70) Lehtola, S.; Tubman, N. M.; Whaley, K. B.; Head-Gordon, M. Cluster Decomposition of Full Configuration Interaction Wave Functions: A Tool for Chemical Interpretation of Systems with Strong Correlation. J. Chem. Phys. **2017**, 147, 154105.
